# Supplementary material for: Spin transport in a magnetic insulator with zero effective damping
Source: arXiv:1812.01334 ancillary file (2019-11-18)
Supplement: Supplementary file 1 [file SI_Spin_transport_in_a_damping_compensated_YIG_film_arxiv_update02.pdf]

# Supplementary Information: Spin transport in a magnetic insulator with zero effective damping

T. Wimmer,[1, 2, *] M. Althammer,[1, 2, †] L. Liensberger,[1, 2] N. Vlietstra,[1]
S. Geprägs,[1] M. Weiler,[1, 2] R. Gross,[1, 2, 3, 4] and H. Huebl[1, 2, 3, 4, ‡]

[1] *Walther-Meißner-Institut, Bayerische Akademie der Wissenschaften, 85748 Garching, Germany*
[2] *Physik-Department, Technische Universität München, 85748 Garching, Germany*
[3] *Nanosystems Initiative Munich (NIM), Schellingstraße 4, 80799 München, Germany*
[4] *Munich Center for Quantum Science and Technology (MCQST), Schellingstr. 4, D-80799 München, Germany*

(Dated: November 18, 2019)

* tobias.wimmer@wmi.badw.de
† matthias.althammer@wmi.badw.de
‡ huebl@wmi.badw.de

# I. SAMPLE LAYOUT

The 13.4 nm thick, single crystalline (100)-oriented yttrium iron garnet ($Y_3Fe_5O_{12}$, YIG) film was grown via pulsed laser deposition at the Walther-Meißner-Institute on a gadolinium gallium garnet ($Gd_3Ga_5O_{12}$, GGG) substrate using a substrate temperature of 450 °C, an oxygen pressure of 25 µbar, a laser fluence at the target of 2.0 J/cm$^2$ and a laser frequency of 10 Hz. The 3.5 nm thick Pt strips were deposited on the YIG thin film by DC sputtering and were patterned by e-beam lithography: the strips have varying edge-to-edge separations $d$ and a constant width of $w$ = 500 nm. The lengths of the Pt strips are $l_{\mathrm{Pt}}$ = 148 µm/162 µm (the middle strips are slightly longer than the outer ones). Subsequently, Ti/Al layers of 5/50 nm were deposited on the film by DC sputtering and patterned into leads for the Pt strips to contact the device electrically. A low frequency ($f$ = 13.131 Hz) AC current $I_{\mathrm{ac}}$ of 50 µA is fed through the injector with a Keithley 6221 current source. To detect the magnon conductivity, we measure the first harmonic SHE voltage $V_{\mathrm{ac}}$ at the detector strip using a Zurich Instruments HF2LI lock-in amplifier. The voltage signal is preamplified by a Stanford Research Systems SR560 low-noise voltage amplifier before being passed to the lock-in. In addition, we vary the DC current $I_{\mathrm{dc}}$ applied to the modulator strip with a Keithley 2400 Sourcemeter to control the magnon chemical potential. The use of this lock-in detection technique is essential to distinguish between magnons stemming from the DC driven modulator and the AC driven injector [S1, S2]. Unless specified otherwise, we will focus on the device with a strip separation of $d$ = 400 nm in this Supplementary Information. An optical micrograph of the device is shown in Fig. S1. For the measurements presented in the main text, the upper middle strip is used as the injector, the lower middle strip as the modulatator and the bottom strip as the detector. For the measurements of the distance dependence and the spin resistance in Sec. VI and VII of this SI, we used the uppermost strip as the injector, while we used the remaining three strips as either detectors or modulators. The measurements are conducted in a cryostat in vacuum at an ambient temperature of $T$ = 280 K. The detector voltage is recorded at constant applied magnetic field as a function of the in-plane angle $\varphi$ between magnetization direction (which is parallel to the applied field at the chosen magnetic field strength) and the Pt strips in a 3D-vector magnet.

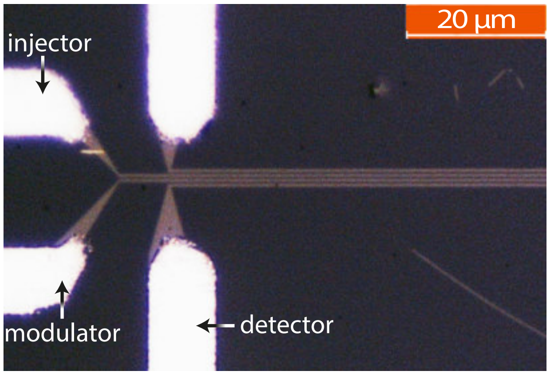


FIG. S1. Optical micrograph of a fraction of a typical device. Black regions correspond to the YIG surface, while the Pt strips appear in dark grey. The strips are contacted with 5 nm/50 nm thick Ti/Al leads (white). In the main text, the strips are used as indicated in the figure. The uppermost strip is only used for measurements of the distance dependence and the spin resistance discussed in Secs. VI and VII.

# II. IN-PLANE FERROMAGNETIC RESONANCE

Since the Gilbert damping $\alpha_{\mathrm{G}}$ of the magnetization dynamics in the YIG film is a crucial parameter in our experiment, we employed in-plane ferromagnetic resonance (FMR) spectroscopy measurements on a bare YIG film with a comparable thickness of 24.5 nm grown with the same parameters by pulsed laser deposition on a (100)-oriented GGG substrate at the Walther-Meißner-Institute. These FMR measurements are performed under ambient conditions (room temperature). In order to measure the spin pumping induced damping $\alpha_{\mathrm{sp}}$, we additionally measured the same YIG film covered with 3.5 nm thick sputtered Pt. To this end, the thin film sample is mounted with the ferromagnetic layer facing the center conductor of a coplanar waveguide (CPW). The complete CPW assembly is placed in the homogeneous magnetic field region of an electromagnet and is connected to a vector network analyzer (VNA). Using the VNA, the complex microwave transmission parameter $S_{21}$ of the setup is measured as a function of the applied magnetic field $\mu_0 H$ and for a series of fixed frequencies $f$ with a fixed microwave power of 1 mW. The resonance fields $\mu_0 H_{\mathrm{res}}$ and linewidths $\mu_0 \Delta H$ are extracted from the real and imaginary part of $S_{21}$ via Lorentzian fits (not shown here).

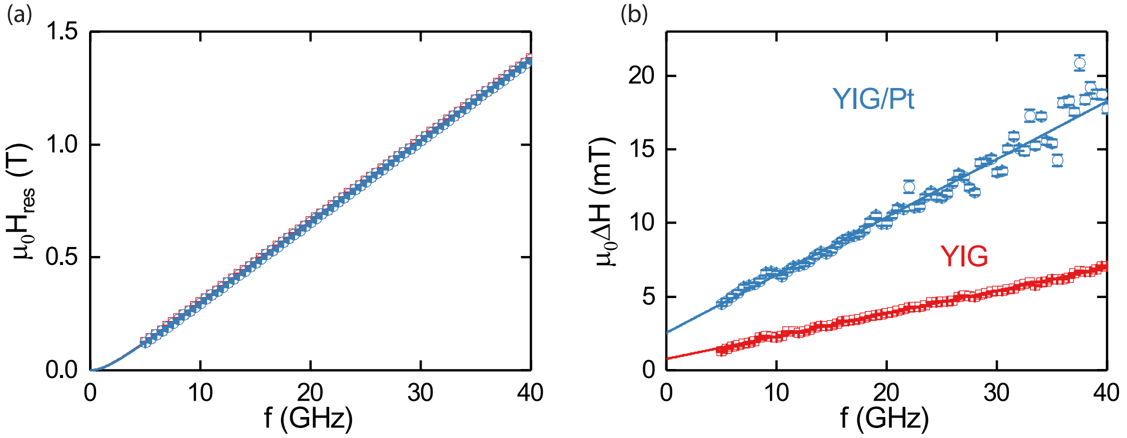


FIG. S2. Ferromagnetic resonance (FMR) data for a 24.5 nm thin YIG film. (a) Frequency dependence of the resonance field for the bare (red data points) and Pt covered YIG film (blue data points). The solid lines are fits by Eq. (S1). (b) Frequency dependence of the FWHM $\mu_0 \Delta H$ of the FMR line for the bare YIG and YIG/Pt film. Solid lines are fits to Eq. (S2).

Fig. S2 (a) shows the frequency dependence of the FMR resonance field for the bare (red data points) and Pt covered YIG film (blue data points) extracted from the Lorentz fits to $S_{21}$. The solid lines are fits to the in-plane Kittel equation

$$f = \frac{\gamma}{2\pi}\mu_0 \sqrt{H_{\mathrm{res}}(H_{\mathrm{res}} + M_{\mathrm{s}})} \tag{S1}$$

with $M_{\mathrm{s}}$ the saturation magnetization of the YIG film and $\gamma = \frac{g\mu_{\mathrm{B}}}{\hbar}$ the gyromagnetic ratio with the Landé factor $g$ and the Bohr's magneton $\mu_{\mathrm{B}}$. The fit results for $M_{\mathrm{s}}$ of the two configurations are shown in Tab. S1. The resonance conditions are not altered for the Pt covered YIG compared to the bare film. As shown in panel (b), however, a significant increase of the full width at half maximum (FWHM) $\mu_0 \Delta H$ is observed when the film is covered with Pt. This is caused by the enhanced Gilbert damping in thin ferromagnetic films covered by normal metals [S3]. The frequency dependence of the linewidth is fitted by

$$\mu_0 \Delta H = \mu_0 \delta H + \frac{4\pi f \alpha_{\mathrm{tot}}}{\gamma} \tag{S2}$$

with fitting parameters $\delta H$ (the inhomogenous FMR linewidth) and $\alpha_{\mathrm{tot}}$ (Gilbert damping), which are also listed in Tab. S1. The difference between the Gilbert damping parameters of the YIG/Pt and the bare YIG film gives the spin pumping induced damping $\alpha_{\mathrm{sp}} = 3.33 \times 10^{-3}$. Since the YIG film studied in the main text is thinner by a factor of $\sim 1.8$ (13.4 nm) compared to the thickness of the film investigated in this section (24.5 nm), we assume an enhanced spin pumping induced damping of $1.8 \cdot \alpha_{\mathrm{sp}} \approx 6 \times 10^{-3}$ in the main text. This is a reasonable assumption due to the reciprocal relation between damping and thickness of the ferromagnetic film [S3]. From the derived $\alpha_{\mathrm{sp}}$, we can calculate the real part of the effective spin mixing conductance as

$$g_{\mathrm{eff}} = \alpha_{\mathrm{sp}} \frac{4\pi M_{\mathrm{s}} t_{\mathrm{YIG}}}{\hbar\gamma}, \tag{S3}$$

giving $g_{\mathrm{eff}} = 7.6 \times 10^{18}\, 1/\mathrm{m}^2$. The spin mixing conductance $g^{\uparrow\downarrow}$ can then be calculated from the experimentally determined $g_{\mathrm{eff}}$ as [S4–S7]

$$g^{\uparrow\downarrow} = g_{\mathrm{eff}} \frac{\frac{h}{e^2}\frac{\sigma_{\mathrm{e}}}{2l_{\mathrm{s}}}}{\frac{h}{e^2}\frac{\sigma_{\mathrm{e}}}{2l_{\mathrm{s}}} - g_{\mathrm{eff}}} \tag{S4}$$

where $e$ is the electron charge, $h$ the Planck constant, $\sigma_{\mathrm{e}}$ denotes the Pt conductivity and $l_{\mathrm{s}}$ the spin diffusion length in Pt. Substituting the corresponding values from Tab. S2, we get $g^{\uparrow\downarrow} = 1.55 \times 10^{19}\, 1/\mathrm{m}^2$. Note, that we assumed the imaginary part of the spin mixing conductance to be zero.

| **bare YIG** (24.5 nm) | Symbol | Value | Unit |
|---|---|---|---|
| saturation magnetization | $\mu_0 M_\mathrm{s}$ | 140 | mT |
| inhomogenous linewidth | $\mu_0 \delta H$ | 0.77 | mT |
| Gilbert damping | $\alpha_\mathrm{tot}$ | $2.17 \times 10^{-3}$ | |
| **Pt covered YIG** | | | |
| saturation magnetization | $\mu_0 M_\mathrm{s}$ | 140 | mT |
| inhomogenous linewidth | $\mu_0 \delta H$ | 2.54 | mT |
| Gilbert damping | $\alpha_\mathrm{tot}$ | $5.50 \times 10^{-3}$ | |

TABLE S1. Values of the fit parameters of Eq. (S1) and (S2) for the bare and Pt covered YIG film.

## III. IMPACT OF THE SPIN SEEBECK EFFECT ON THE CRITICAL CURRENT

The spin Seebeck effect (SSE) due to the current-heating in our experiment was not taken into account in Eq. (1) of the main text (see also Sec. X). The SSE is driven by the temperature difference $\delta T$ between the electron and the magnon system at the ferromagnetic insulator/normal metal interface [S8] arising from the Joule heating of the Pt strips. According to Bender et al. [S9], this temperature difference $\delta T$ between the electron system in Pt and magnon system in YIG causes a vertical offset of the BEC threshold $\mu_{c=2}$ due to the spin injection driven by $\delta T$[S10]. In order to estimate the magnitude of this effect, SSE measurements allowing to determine $\delta T$ are necessary. Hence, we evaluate the temperature difference experimentally via the SSE at the modulator strip for a heating current of 0.55 mA. To this end, we measured the thermal contribution of the voltage drop $V_\mathrm{Therm}$ across the modulator strip as a function of the magnetic field orientation $\varphi$ at $\mu_0 H = 50\,\mathrm{mT}$, as shown in Fig. S3. The amplitude of the modulation is then extracted by fitting a sinusoidal function to the measured $V_\mathrm{Therm}$ $(\varphi)$ dependence. The amplitude of this sinusoidal function is obtained to $A_\mathrm{SSE} \approx 3.24\,\mathrm{mV}$. The spin Seebeck voltage is then $V_\mathrm{SSE} = \frac{A_\mathrm{SSE}}{2} = 1.62\,\mathrm{mV}$. Theoretically, we can calculate $\delta T_\mathrm{SSE}$ via [S8, S11]

$$V_\mathrm{SSE} = \frac{g^{\uparrow\downarrow}\gamma\hbar k_\mathrm{B}}{2\pi M_\mathrm{s} V_\mathrm{a}} \cdot \delta T_\mathrm{SSE} \cdot \frac{2e}{\hbar\sigma_\mathrm{e}} l_\mathrm{Pt} \cdot \xi \cdot \frac{l_\mathrm{s}}{t_\mathrm{Pt}} \tanh\left(\frac{t_\mathrm{Pt}}{2l_\mathrm{s}}\right) \tag{S5}$$

with a backflow correction factor $\xi = \left[1 + 2g^{\uparrow\downarrow} l_\mathrm{s} \frac{e^2}{\hbar\sigma_\mathrm{e}} \coth\left(\frac{t_\mathrm{Pt}}{l_\mathrm{s}}\right)\right]^{-1}$ and the magnetic coherence volume $V_\mathrm{a} =$

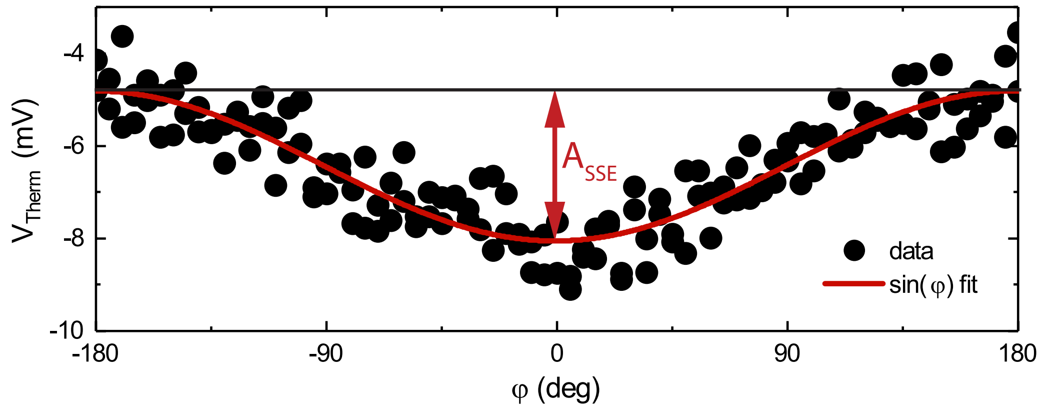


FIG. S3. Spin Seebeck contribution to the voltage drop across the modulator strip as a function of the magnetic field orientation $\varphi$ for a heating current of 0.55 mA and an applied magnetic field magnitude of $\mu_0 H = 50\,\mathrm{mT}$. The amplitude $A_\mathrm{SSE}$ is extracted as the amplitude of the sinusoidal fit.

$\frac{2}{3\zeta(5/2)}\left(\frac{4\pi J_\mathrm{s}}{k_\mathrm{B} T}\right)^{3/2}$ [S8, S11]. Finally, we find an experimentally determined temperature difference via the SSE voltage of $\delta T_\mathrm{SSE} = 0.14\,\mathrm{K}$, corresponding to a thermal energy of $k_\mathrm{B}\delta T = 12\,\mathrm{\mu eV}$. Comparing this to Fig. 6 in Ref. [S9], the SSE is found to only marginally affect the threshold condition for the BEC phase transition (for the swasing phase transition there is no effect at all). An estimate of the enhancement of the critical current due to the thermally injected magnons from Ref. [S9] gives roughly $\sim 3\,\mathrm{\mu A}$ for $\delta T_\mathrm{SSE} = 0.14\,\mathrm{K}$, which is smaller than 1 % of the typical

critical currents found in this experiment ($I_{on/crit} \approx 500\,\mu A$). Hence, the current-induced heating of the Pt strip does not cause a measurable impact on $I_{on/crit}$ in our experiments.

## IV. LOCAL THERMOMETRY

The current densities applied to the DC modulator strip range up to almost $4.6 \times 10^{11}\,A/m^2$ (for the highest current value of $I_{dc} = 0.8\,mA$ used in this work). The total resistance of the modulator strip at $T = 280\,K$ is approximately $50\,k\Omega$, resulting in a power density of almost $\sim 40\,kW/cm^2$. Due to this large Joule heating present in our sample, we performed thermometry measurements by measuring the Pt resistance to characterize the actual temperature increase of the device. To this end, we applied a small DC current of $10\,\mu A$ to the three strips (injector, modulator and detector) and measured the respective voltages as a function of the base temperature of the cryostat. The resulting resistance vs. temperature curves of the strips are shown in Fig. S4 (a) and can be viewed as calibration curves of Pt thermometers. As expected for metals, a linear increase of the resistivity with increasing temperature is observed. Subsequently, we swept the modulator current from $-0.8\,mA$ to $0.8\,mA$ for a base temperature of $T = 280\,K$ (which is equal to the base temperature used in the measurements in the main text) while applying a small current of $10\,\mu A$ to the injector and detector electrodes. The measured local temperatures as a function of the modulator current are plotted in Fig. S4 (b). Evidently, at the maximum modulator current of $0.8\,mA$ the associated Joule heating results in a temperature increase at the modulator up to is $370\,K$. However, at this temperature YIG can still be considered as a good electrical insulator [S12]. We therefore exclude spurious electrical crosstalk effects as a possible origin of our all-electrical magnon transport signals. The injector and detector strips only reach temperatures up to $330\,K$. Note, that the temperature of the modulator strip does not reach the base temperature of $280\,K$ for zero modulator current, which is most probably due to an incomplete thermalization of the modulator strip during the current sweep.

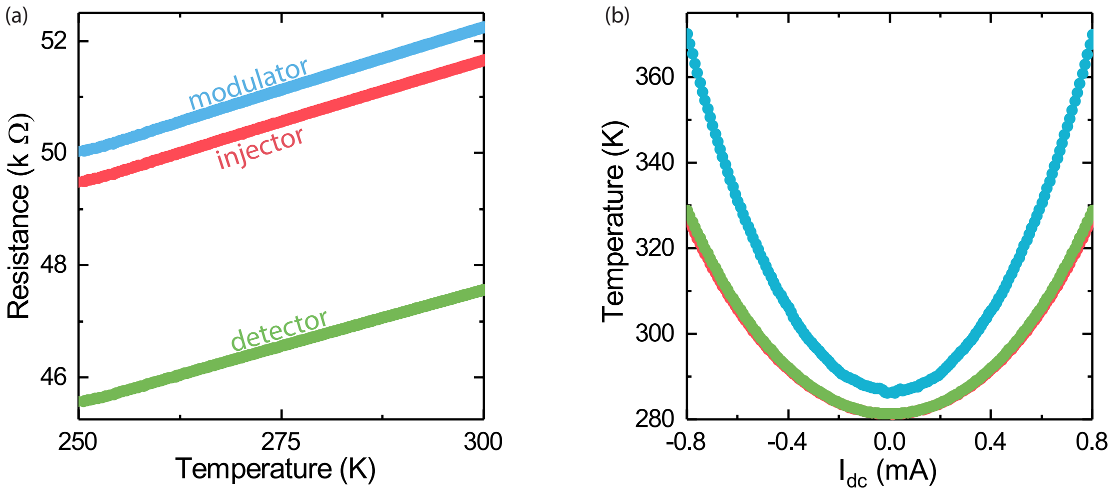


FIG. S4. (a) Resistance of injector, modulator and detector as a function of the base temperature of the sample. The linear dependencies are used as calibration curves, allowing to use the strips as local temperature sensors. (b) DC current dependence of the temperature in the three Pt strips.

We also investigated the electrical isolation between injector and detector as a function of the modulator current. Over the whole current range the resistance between injector and detector is above $1\,G\Omega$, which is 5 orders of magnitude larger than the Pt resistance and comparable to the input resistance of the measurement setup, such that any influence from enhanced electrical conduction from the YIG layer can be ruled out in our experiments.

## V. SPIN HALL EFFECT AND THERMALLY INDUCED MODULATION OF THE MAGNON CONDUCTIVITY

The $A(I_{dc})$ curves shown in Fig. 3 in the main text contain contributions due to both the SHE and temperature gradients generated by Joule heating in the modulator. Fortunately, we can distinguish between the two contributions according to their symmetries: the SHE contribution is odd, while the thermal contribution is even in the field direction. Therefore, we extract the modulation amplitude due to the SHE by calculating the antisymmetric part

of the amplitudes as $A_{\mathrm{SHE}} = \frac{A(+\mu_0 H) - A(-\mu_0 H)}{2}$ and the thermal contribution as the symmetric part as $A_{\mathrm{Therm}} = \frac{A(+\mu_0 H) + A(-\mu_0 H)}{2}$. We then normalize $A_{\mathrm{SHE}}$ and $A_{\mathrm{Therm}}$ leading to

$$\eta_{\mathrm{SHE}} = \frac{A_{\mathrm{SHE}}}{A_{\mathrm{I_{dc}}=0}} = \frac{\sigma_{\mathrm{m}}^{\mathrm{SHE}}}{\sigma_{\mathrm{m}}^{0}} \tag{S6a}$$

$$\eta_{\mathrm{Therm}} = \frac{A_{\mathrm{Therm}} - A_{\mathrm{I_{dc}}=0}}{A_{\mathrm{I_{dc}}=0}} = \frac{\sigma_{\mathrm{m}}^{\mathrm{Therm}}}{\sigma_{\mathrm{m}}^{0}} \tag{S6b}$$

with $A_{\mathrm{I_{dc}}=0}$ the detector amplitude at zero DC modulation current. The relative modulation strength $\eta_{\mathrm{SHE}}$ ($\eta_{\mathrm{Therm}}$) is then proportional to the ratio of the SHE (thermally) induced magnon conductivity $\sigma_{\mathrm{m}}^{\mathrm{SHE}}$ ($\sigma_{\mathrm{m}}^{\mathrm{Therm}}$) and the magnon conductivity in thermal equilibrium $\sigma_{\mathrm{m}}^{0}$ [S2].

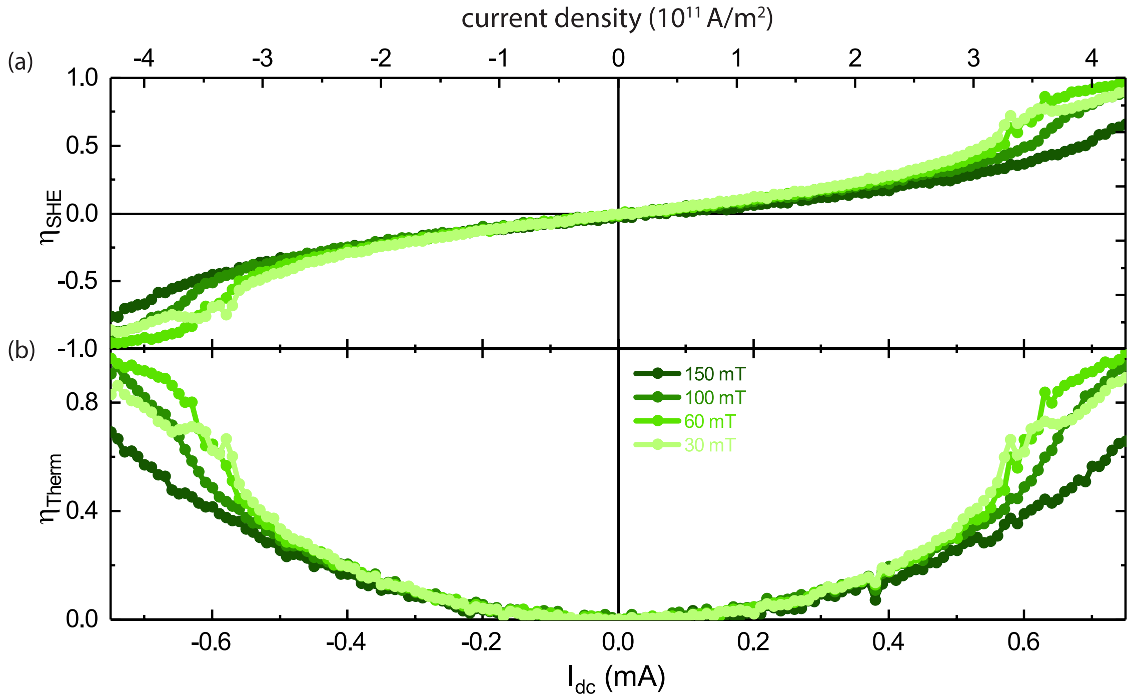


FIG. S5. (a) Spin Hall effect induced relative modulation strength $\eta_{\mathrm{SHE}}$ calculated from the experimental data using Eq. (S6a). (b) Thermally induced modulation $\eta_{\mathrm{Therm}}$ calculated using Eq. (S6b).

Fig. S5 (a) shows $\eta_{\mathrm{SHE}}$ as a function of the DC current. For small currents ($|I_{\mathrm{dc}}| \lesssim 0.4\,\mathrm{mA}$), a linear regime is observed. This behaviour is expected for the SHE induced modulation as long as the magnon chemical potential does not reach the magnon gap energy, such that the magnon excitation is restricted to the thermally excited magnon spectrum [S13]. For $|I_{\mathrm{dc}}| \gtrsim 0.4\,\mathrm{mA}$, the SHE modulation becomes non-linear. Furthermore, the peak/kink structure indicating the damping compensation is clearly observed. Panel (b) shows the thermally induced relative modulation strength $\eta_{\mathrm{Therm}}$ as a function of the DC current. Here, the small current regime follows a quadratic dependence with the applied DC current, which is expected for the thermal injection of magnons. For larger currents, the threshold behaviour is again evident.

The quantitative agreement between theoretical prediction and experimental data regarding the field dependent threshold condition (parametrized by the critical currents $I_{\mathrm{on}}$, $I_{\mathrm{crit}}$) shown in Fig. 4 (a) in the main text could be explained by the presence of the Bose-Einstein condensation of magnons. In particular, the phase transition is expected to follow the magnetic field dependence given by Eq. (1) in the main text (see also Eq. (S22) in Sec. X). In order to verify this as a unique feature, we evaluate the field dependence of the modulation efficiency within the linear regime of the $\eta_{\mathrm{SHE}}$ dependence shown in Fig. S5 (a). The modulation efficiency is evaluated as the slope of $\eta_{\mathrm{SHE}}$ by linearly fitting the data within the current range of $|I_{\mathrm{dc}}| < 0.4\,\mathrm{mA}$. The result is shown in Fig. S6, where the efficiency is plotted in units of %/mA versus the applied magnetic field. Clearly, we observe a qualitatively different field dependence as compared to that of Eq. (1) of the main text that we found for the magnon BEC/swasing phase state. Instead, the observed field dependence is similar to the usual magnetic field dependence observed for thermal magnon transport [S14].

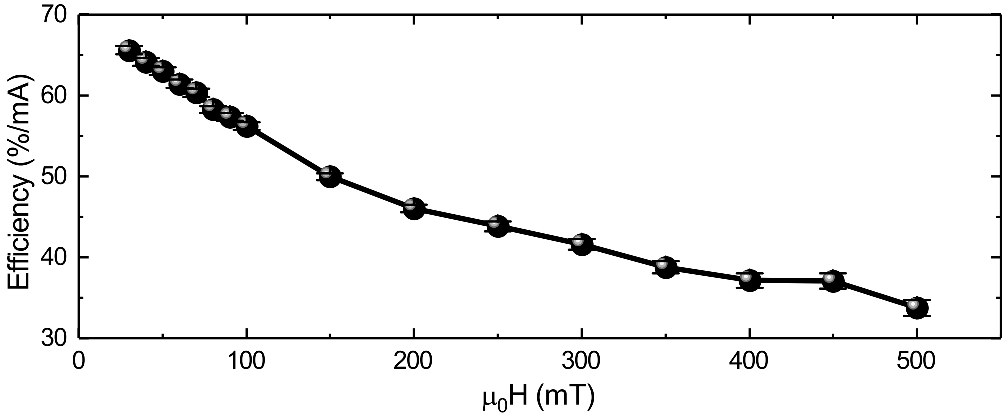


FIG. S6. Spin Hall effect induced efficiency in units of %/mA as a function of the applied magnetic field. The field dependence is qualitatively different from the field dependence of the critical current in Fig. 4 (b) of the main text.

As predicted in Ref. S2, the modulation efficiency for 10 nm thin YIG films at $\mu_0 H = 50\,\mathrm{mT}$ is expected to be about $\sim 16\,\%/\mathrm{mA}$. The YIG thin film in this study with $t_{\mathrm{YIG}} = 13.4\,\mathrm{nm}$, however, shows a significantly larger efficiency of $\sim 60\,\%/\mathrm{mA}$ at $\mu_0 H = 50\,\mathrm{mT}$, which exceeds the prediction by a factor of $\sim 4$. Thus, our results show that thermal magnon based logic is even more efficient in very thin YIG films than theoretically expected.

## VI. MEASUREMENTS AS A FUNCTION OF INJECTOR-DETECTOR SEPARATION

In this Section, we focus on the study of magnon transport as a function of the injector-detector separation. This study is performed both within and outside of the damping compensated regimes. These measurements were performed on two devices each containing a four-strip structure with edge-to-edge distances of $d = 400\,\mathrm{nm}$ and $d = 200\,\mathrm{nm}$ for a fixed magnetic field of $\mu_0 H = 50\,\mathrm{mT}$. Here, we apply an AC current to the injector, while we use the three remaining strips as detectors (as shown in the inset in Fig. S7 (a), denoted as 'inj', 'det 1', 'det 2' and 'det 3'). The amplitudes $A$ of the first harmonic magnon transport signal as a function of the edge-to-edge distances $d$ between injector and detectors are shown in Fig. S7a and b (red open circles). We observe an exponential decrease of the signal, which is expected for diffusive magnon transport [S15]. A simple exponential fit (red line) gives a magnon diffusion length of $\lambda_{\mathrm{m}} = 1.09\,\mu\mathrm{m} \pm 0.08\,\mu\mathrm{m}$. Subsequently, we measure the distance dependence while applying a DC modulation current $I_{\mathrm{dc}}$ to a modulator strip (detector 1 is now used as a DC modulator) for the case when the DC current *increases* the magnon conductivity (see Fig. 2 in the main text). At this point, we have to distinguish two current regimes: first, below the damping compensation ($I_{\mathrm{dc}} < I_{\mathrm{on}}$) we expect to have a increase of magnon conductivity due to the magnon density increase (SHE and thermal injection of magnons), while for $I_{\mathrm{dc}} > I_{\mathrm{crit}}$ we expect an additional increase of the magnon conductivity due to the damping compensation. In order to separate the contribution below the compensation from the one beyond, we calculate a corrected signal amplitude

$$A_{\mathrm{corr}} = A - [A_{\mathrm{SHE}} + (A_{\mathrm{Therm}} - A_{\mathrm{I_{dc}=0}})] \tag{S7}$$

where the contribution below the compensation is subtracted. For $I_{\mathrm{dc}} < I_{\mathrm{on}}$, this is done by taking the amplitudes $A_{\mathrm{SHE}}$ and $A_{\mathrm{Therm}} - A_{\mathrm{I_{dc}=0}}$ (see Sec. V) stemming from the SHE and thermally induced magnon injection and subtract these from the measured amplitudes $A$. For $I_{\mathrm{dc}} > I_{\mathrm{on}}$, however, $A_{\mathrm{SHE}}$ ($A_{\mathrm{Therm}}$) deviates significantly from a simple linear (quadratic) behaviour (see Fig. S5). We therefore extrapolate them linearly (quadratically) into the high current regime and then use the extrapolated values to correct the amplitudes in this high current regime. We hereby isolate the effect of the critical behaviour on the magnon transport properties. Note, that for $I_{\mathrm{dc}} = 0$ the corrected amplitudes $A_{\mathrm{corr}}$ are equal to the raw signal amplitudes $A$.

We start with the regime below compensation by applying a current of $I_{\mathrm{dc}} = 0.4\,\mathrm{mA} < I_{\mathrm{on}}$ to one modulator and measure the signals at detector 2 and 3. The resulting $A_{\mathrm{corr}}$ is plotted as a function of distance in Fig. S7 (a) (blue open triangles). As expected, the amplitudes $A_{\mathrm{corr}}$ perfectly match the ones obtained without applied modulation current. Subsequently, we repeat the distance dependent measurements for a modulation current $I_{\mathrm{dc}} = 0.6\,\mathrm{mA} > I_{\mathrm{crit}}$ to get information on the magnon transport within damping compensated regime and compute $A_{\mathrm{corr}}$ shown as dark blue open stars. Obviously, the corrected amplitudes are now remarkably larger than for the non-compensated case. An exponential fit to these points gives $\lambda_{\mathrm{m}} = 0.96\,\mu\mathrm{m} \pm 0.01\,\mu\mathrm{m}$, which is in good agreement with the diffusion

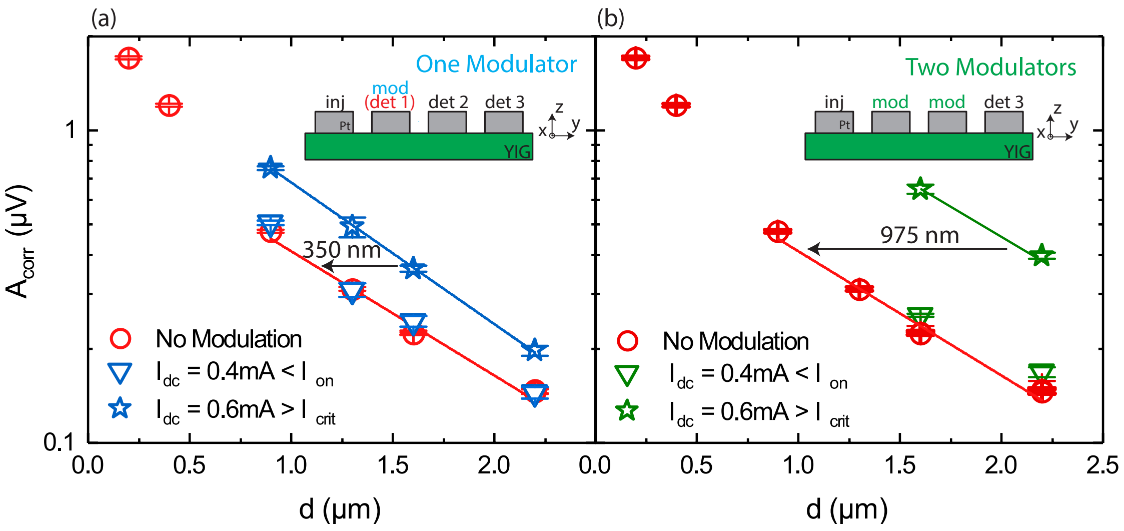


FIG. S7. Magnon transport signal amplitudes $A_{\mathrm{corr}}$ as a function of the distance $d$ between injector and detector. Note, that the contribution to the increase of the magnon conductivity below the damping compensation is subtracted. Red data points show the distance dependence when no DC modulation current is applied, including an exponential fit to the data for $d \geq 0.9\,\mu\mathrm{m}$ (red line). (a) The blue data points show the corrected signal amplitudes for a single DC modulation strip as indicated in the inset. While the corrected signals are unchanged for $I_{\mathrm{dc}} = 0.4\,\mathrm{mA} < I_{\mathrm{on}}$ (blue triangles), there is a remarkable increase in signal for $I_{\mathrm{dc}} = 0.6\,\mathrm{mA} > I_{\mathrm{crit}}$ (blue stars), which is also fitted with an exponential fit (blue line) for the same region. When shifting the blue line by 350 nm to the left, the same distance dependence as for the non-modulated case is observed, hence indicating zero resistance transport within a path of 350 nm length. (b) The green data points (triangles and stars) show the distance dependence within and outside of the damping compensated state for the case when two strips are simultaneously biased with a DC modulator current as indicated in the inset. Here, zero resistance magnon transport is found to occur over a distance of 975 nm.

length for the non-modulated case. Hence, the distance dependence within the damping compensated regime is only altered regarding its amplitudes. The entire decay curve seems to be shifted to larger distances indicating that the characteristic magnon transport length is not affected and that the transport beneath the strips seems to be without resistance. This allows to estimate the extension of the damping compensated region in the YIG by comparing the distance dependence measured above compensation ($I_{\mathrm{dc}} > I_{\mathrm{crit}}$, blue stars) with the one measured below ($I_{\mathrm{dc}} < I_{\mathrm{on}}$, blue triangles). The shift in $d$ between the red data and the dark blue data is about 350 nm. Thus, the data indicates that we observe about 350 nm of zero resistance magnon transport. This also suggest that the zero damping regime is located just underneath the modulator strip with a width of $w = 500\,\mathrm{nm}$.

In a second experiment, we simultaneously bias two DC modulators with a current of the same magnitude and polarity, while measuring the first harmonic transport signal at detector 3 for both devices (see inset in Fig. S7 (b)). Similar to the case for one modulator, we measure the magnon transport signal for $I_{\mathrm{dc}} = 0.4\,\mathrm{mA} < I_{\mathrm{on}}$ (outside the compensated regime) and $I_{\mathrm{dc}} = 0.6\,\mathrm{mA} > I_{\mathrm{crit}}$ (within the compensated regime), which we apply to both modulators simultaneously. This is shown in Fig. S7 (b), where the corrected amplitudes $A_{\mathrm{corr}}$ at detector 3 are plotted for $I_{\mathrm{dc}} = 0.4\,\mathrm{mA}$ (green triangels) and $I_{\mathrm{dc}} = 0.6\,\mathrm{mA}$ (green stars). The data points for $I_{\mathrm{dc}} < I_{\mathrm{on}}$ match the ones without $I_{\mathrm{dc}}$ applied to the modulator reasonably. For $I_{\mathrm{dc}} > I_{\mathrm{crit}}$, the signals are again significantly larger in amplitude. Here, the green stars indicate a shift of the curve by 975 nm, therefore implying a lateral extension of the damping compensated region of $\sim$ 975 nm. Naively, one would expect the extension of this region to scale linearly with the effective modulator width, suggesting an extension twice as large as estimated for the case with a single modulator. Evidently, this is not the case in our experiment. Since, however, the overall magnon density underneath the two modulators is mutually increased, the critical magnon density required for the damping compensation is expected to be accessible for smaller DC currents in the modulators. Therefore, the extension of the damping compensated region is actually expected to increase by a factor of more than 2 when two seperate modulators are used.

## VII. SPIN RESISTANCE IN YIG

The spin resistance $R^{\mathrm{s}}_{\mathrm{YIG}}$ in YIG is determined by adopting an equivalent spin resistor model for our device from Ref. S16, according to which

$$R^{\mathrm{s}}_{\mathrm{YIG}} = \frac{R^{\mathrm{s}}_{\mathrm{Pt}}}{\eta_{\mathrm{s}}} - (2R^{\mathrm{s}}_{\mathrm{int}} + 2R^{\mathrm{s}}_{\mathrm{Pt}}) \tag{S8}$$

where $R^{\mathrm{s}}_{\mathrm{Pt}} = l_{\mathrm{s}}/(\sigma_{\mathrm{e}} A_{\mathrm{int}} \tanh(t_{\mathrm{Pt}}/l_{\mathrm{s}}))$ is the spin resistance of the Pt strip and $R^{\mathrm{s}}_{\mathrm{int}} = 1/(g_{\mathrm{s}} A_{\mathrm{int}})$ the interface spin resistance. In the following, we will neglect the last to terms in Eq. (S8) (i.e. the interface and Pt spin resistances), since these are three orders of magnitude smaller than the first term. $\eta_{\mathrm{s}}$ denotes the spin transfer efficiency from injector to detector and reads

$$\eta_{\mathrm{s}} = \frac{t_{\mathrm{Pt}}}{l_{\mathrm{s}}\theta^2_{\mathrm{SH}}} \frac{A_{\mathrm{corr}}}{I_{\mathrm{ac}} R_{\mathrm{det}}} \frac{(e^{t_{\mathrm{Pt}}/l_{\mathrm{s}}} + 1)(e^{2t_{\mathrm{Pt}}/l_{\mathrm{s}}} + 1)}{(e^{t_{\mathrm{Pt}}/l_{\mathrm{s}}} - 1)^3} \tag{S9}$$

with $R_{\mathrm{det}}$ the resistance of the Pt detector strip. In order to isolate the effect of the damping compensation on the spin resistance, we use the corrected voltage amplitudes $A_{\mathrm{corr}}$ of the magnon transport signal for the calculation of $\eta_{\mathrm{s}}$ (see Sec. VI) and eventually of $R^{\mathrm{s}}_{\mathrm{YIG}}$.

As done in the previous Section, we investigate two different measurement configurations (compare Sec. VI): first, we use the outermost Pt strip as the AC injector, the neighbouring strip as the DC modulator and the remaining strips as detectors (denoted as 'inj', 'mod', 'det 2' and 'det 3' in the inset scheme in Fig. S8 (b)). In the second configuration, we use the two middle strips of the four strip devices as DC modulators, while we measure the magnon transport signal at detector 3 (see inset in Fig. S8 (c)). The two modulators are simultaneously biased with currents of the same magnitude and polarity.

We start with the first configuration, where we use only a single modulator. In Fig. S8 (a) and (b) the spin resistance $R^{\mathrm{s}}_{\mathrm{YIG}}$ is evaluated from the signal amplitude at detector 2 and 3 as a function of the DC current in the modulator for a positive magnetic field $\mu_0 H = 50\,\mathrm{mT}$ (positive field corresponds to the $-\mathbf{y}$-direction). Black data points represent the results for the device with an edge-to-edge distance of $d = 400\,\mathrm{nm}$, while the orange ones stand for the device with $d = 200\,\mathrm{nm}$. The parameter $d_{\mathrm{inj-det}}$ denotes the effective distance between the AC injector and the respective detector. Due to the positive magnetic field that we apply in this measurement, positive DC currents correspond to magnon injection ($I_{\mathrm{dc}}$ along $\mathbf{x}$-direction), while negative currents correspond to magnon depletion ($I_{\mathrm{dc}}$ along $-\mathbf{x}$-direction). In the magnon injection regime ($I_{\mathrm{dc}} > 0$), we observe a steep decrease of the spin resistance around the critical current for both detectors, indicating the BEC phase transition. The magnon depletion regime ($I_{\mathrm{dc}} < 0$) shows a constant spin resistance up to $I_{\mathrm{dc}} = -0.4\,\mathrm{mA}$. An increase of the spin resistance is observed for $I_{\mathrm{dc}} < -0.4\,\mathrm{mA}$. Since we used the corrected amplitudes $A_{\mathrm{corr}}$ for the calculation of the spin resistance, we expect no effect of the linear SHE induced and quadratic thermally induced contribution to the magnon conductivity modulation. We therefore infer that other non-linear effects regarding the SHE induced depletion of the magnon system increase the spin resistance in this regime [S17].

Measurements in the second configuration using two modulators are shown in Fig. S8 (c) with the insets showing a zoom into the regime for $I_{\mathrm{dc}} > 0$ and a schematic of the measurement configuration. Similar to the case using a single modulator, the transition into the zero damping state, indicated by the drop in spin resistance for $I_{\mathrm{dc}} > I_{\mathrm{on}}$, is still evident. The non-linear increase of spin resistance for negative modulator currents ($I_{\mathrm{dc}} < -0.4\,\mathrm{mA}$) is even more pronounced than for the result obtained with a single modulator strip. Since we attributed this increase to non-linear effects regarding the depletion of the magnon system, we do expect this effect to be larger when two modulators are used due to the aforementioned mutual modulation (in this case: decrease) of magnon density beneath each strip.

To estimate the spin resistivity in the zero damping state $\rho^{\mathrm{s}}_{\mathrm{YIG,crit}}$, we first calculate the spin resistivity $\rho^{\mathrm{s}}_{\mathrm{YIG,NC}}$ in the normal phase for the detector with $d_{\mathrm{inj-det}} = 1.3\,\mu\mathrm{m}$ (Fig. S8 (a), black symbols). In doing so, we take the average spin resistance $R^{\mathrm{s}}_{\mathrm{YIG,NC}}$ for the current range $0 < I_{\mathrm{dc}} < 0.4\,\mathrm{mA}$ and then calculate $\rho^{\mathrm{s}}_{\mathrm{YIG,NC}} = R^{\mathrm{s}}_{\mathrm{YIG,NC}} t_{\mathrm{YIG}} l_{\mathrm{Pt}}/d_{\mathrm{inj-det}}$ and obtain $\rho^{\mathrm{s}}_{\mathrm{YIG,NC}} = 0.54(8)\,\mu\Omega\,\mathrm{m}$. In a similar fashion, we determine the average spin resistance $R^{\mathrm{s}}_{\mathrm{YIG,crit}}$ for the current range $0.6\,\mathrm{mA} \leq I_{\mathrm{dc}} \leq 0.8\,\mathrm{mA}$ in the damping compensated regime. To estimate the spin resistivity in the compensated region, we assume that it extends for $d_{\mathrm{crit}} = 540\,\mathrm{nm}$ in $\mathbf{y}$-direction underneath the modulator. Further assuming that the resistivity in the normal phase has not changed and a simple series resistor model can be applied in the spin resistance network, we calculate $\rho^{\mathrm{s}}_{\mathrm{YIG,crit}} = \left(R^{\mathrm{s}}_{\mathrm{YIG,crit}} - \frac{d_{\mathrm{inj-det}} - d_{\mathrm{crit}}}{d_{\mathrm{inj-det}}} R^{\mathrm{s}}_{\mathrm{YIG,NC}}\right) t_{\mathrm{YIG}} l_{\mathrm{Pt}}/d_{\mathrm{crit}}$ and obtain $\rho^{\mathrm{s}}_{\mathrm{YIG,crit}} = 8.16(79)\,\mathrm{n}\Omega\,\mathrm{m}$. Again, this strong reduction of spin resistivity by almost two orders of magnitude indicates zero resistance magnon transport within the damping compensated region. Note, however, that this crude estimation strongly depends on the value of $d_{\mathrm{crit}}$. We therefore extracted the value of $d_{\mathrm{crit}}$ (i.e. the width of the modulator strip) from atomic force microscopy (AFM) measurements, which are shown in Fig. S9 (a) and (c). Since the sample was glued to a carrier for the transport measurements, it had to be removed from the carrier for the AFM measurements, resulting in the reduced image quality of the sample discussed in the main text, as shown in Fig. S9 (c). Nevertheless, all of the devices on the sample have equal strip widths of 500 nm defined by electron beam lithography. We therefore

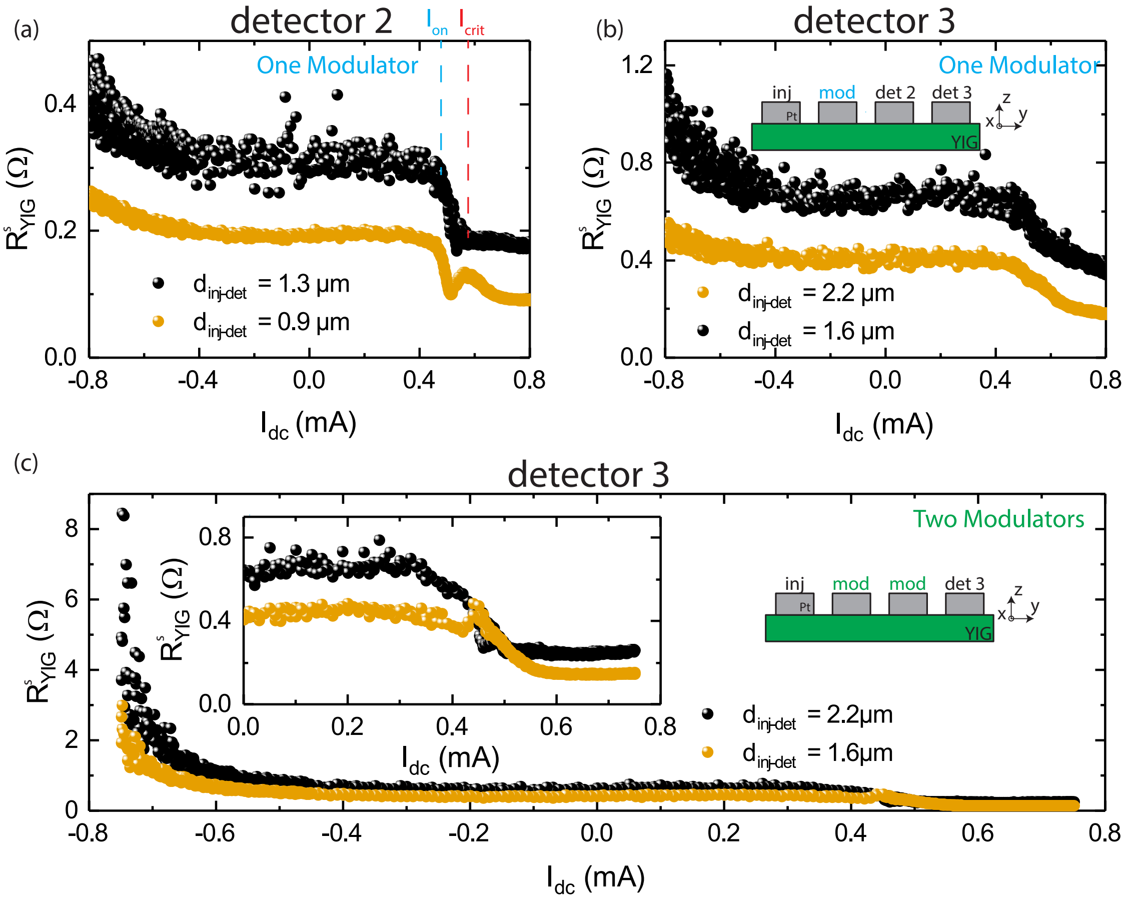


FIG. S8. Calculated spin resistance $R^{\mathrm{s}}_{\mathrm{YIG}}$ as a function of the modulator current $I_{\mathrm{dc}}$ at 280 K and $\mu_0 H = 50\,\mathrm{mT}$. The upper panels (a) and (b) show the YIG spin resistances evaluated from the magnon transport signals measured at detector 2 and 3, respectively (shown for both investigated devices, represented by black and orange data points). A steep decrease of the spin resistance is oberved when $I_{\mathrm{dc}} > I_{\mathrm{crit}}$, while a slight increase in spin resistance is observed for $I_{\mathrm{dc}} < -0.4\,\mathrm{mA}$. (c) $R^{\mathrm{s}}_{\mathrm{YIG}}$ calculated from measurements with two modulator strips and detection on detector 3 for the two devices investigated. Once again, a steep decrease in resistance is obtained for $I_{\mathrm{dc}} > I_{\mathrm{crit}}$, as well as a rather large increase in spin resistance for $I_{\mathrm{dc}} < -0.4\,\mathrm{mA}$. The inset shows an enlarged view of the positive current regime.

measured a similar structure on the same sample using the AFM in Fig. S9 (a). Here, a device with strip distances of $d = 800\,\mathrm{nm}$ is shown. To determine the strip width, we plot line cuts at four different positions perpendicular to the strips (see red lines in Fig. S9 (a)). The corresponding line scans are shown in Fig. S9 (b). We then extract the strip width by measuring the distance between each of the edges corresponding to the borders of the strips (we here take the middle of the edge flanks as the markers for measuring the distance, as shown by the black vertical lines in Fig. S9 (b)). In doing so, we find for the strip widths determined by the AFM from left to right: $w_{\mathrm{AFM}}$ =560 nm, 500 nm, 550 nm, 560 nm, while the strip distances are: $d_{\mathrm{AFM}}$ = 780 nm, 830 nm, 800 nm, 560 nm. Hence, we indeed find that the strip widths commonly exhibit a slightly larger value than defined by the electron beam lithography [S18]. The AFM measurements of the device presented in the main text still allow to resolve the strips, as seen in Fig. S9 (c). Here, we measured the strip width of the modulator via the 2D scan. As shown by the red line labelled with '1' in Fig. S9 (c), the modulator width indeed exhibits a width of 540 nm, which is in perfect agreement with the value of $d_{\mathrm{crit}}$ assumed above. Hence, resukting in the calculated value of the spin resistivity $\rho^{\mathrm{s}}_{\mathrm{YIG,crit}} = 8.16(79)\,\mathrm{n}\Omega\,\mathrm{m}$. In the experiment, however, one will be ultimately limited by the finite spin resistance contributions from the interface ($R^{\mathrm{s}}_{\mathrm{int}}$) and the Pt injector/detector ($R^{\mathrm{s}}_{\mathrm{Pt}}$), which we have not accounted for in this estimation.

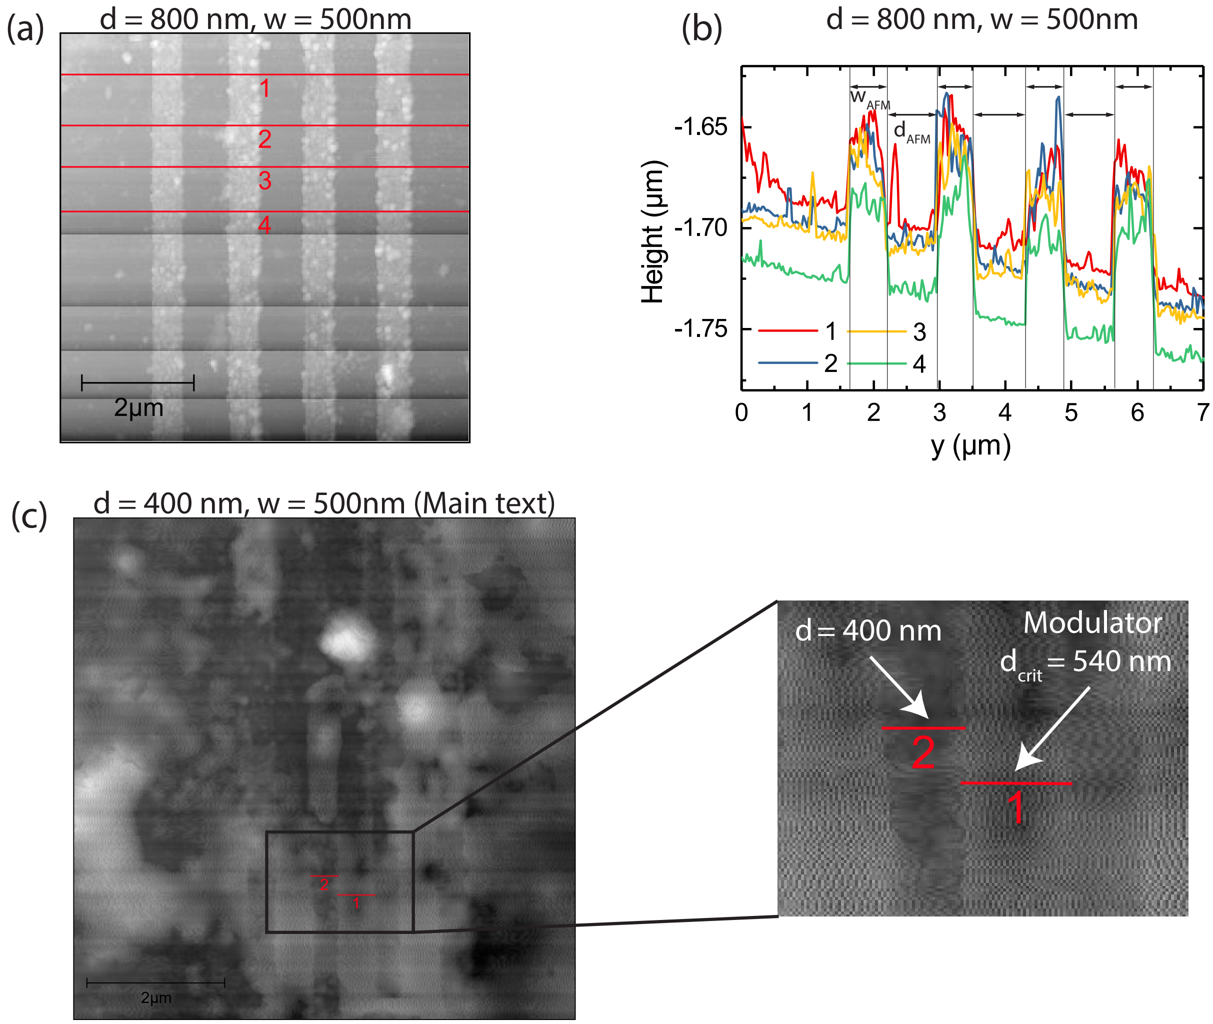


FIG. S9. (a) 2D AFM scan of a device with strip distance $d = 800\,\mathrm{nm}$ and widths $w = 400\,\mathrm{nm}$. The strips are shown as the light grey areas. The red lines represent the line cuts, which are plotted in (b).From the line cuts, the strip widths and distances are extracted by measuring the distance between each of the vertical black marker lines drawn in the plot. The marker lines were set at the middle of each of the steep edges in the line scan. (c) 2D AFM scan of the device studied in the main text. Due to surface contaminations present on the device, the strips are less clearly visible. Still, the strip width of the modulator was extracted via measuring the distance between the edges of the strip on the 2D scan (red line labelled '1'). Here, we find a width of 540 nm, which corresponds well to the value of $d_{\mathrm{crit}}$ assumed for the extension of the damping compensated regime beneath the modulator. In order to verify that the device shows the expected strip separation, this was also measured in the 2D scan (line labelled by '2').

## VIII. IMPACT OF MAGNETOCRYSTALLINE ANISOTROPY AND THE CRITICAL MAGNON CONDUCTIVITY ENHANCEMENT ON ANGULAR DEPENDENT MEASUREMENTS

In this Section, we quantitatively investigate the impact of the cubic magnetocrystalline anisotropy of YIG as well as the influence of the DC current in the modulator on the shape of the angle dependent magnon transport measurements. We first start with the angle dependent measurement for $I_{\mathrm{dc}} = 0\,\mu\mathrm{A}$ shown in Fig. 2 of the main text, which is shown again in Fig. S10 (a) for convenience (black data points). It is obvious, that the measurement displays a rather triangular shape compared to the expected $\cos^2(\varphi)$-like modulation, which is shown as a fit to the data (blue solid line) in Fig. S10 (a). This discrepancy stems from the in-plane cubic anisotropy of our (100)-oriented YIG film, leading to a slight misalignment of the external field direction $\varphi$ and the magnetization direction $\varphi_{\mathrm{m}}$ of the YIG film. Since the data is measured for an external field of $\mu_0 H = 50\,\mathrm{mT}$ , a visible contribution of the anisotropy to the angular dependent meaurements is likely. In order to quantitatively model this behaviour, we implement the cubic anisotropy by introducing a Stoner-Wohlfarth-model as

$$f(\varphi_{\rm m}) = -\mu_0 \mathbf{H}\cdot\mathbf{M} + K_{\rm c1} m_{\rm x}^2 m_{\rm y}^2. \tag{S10}$$

Here, $f$ is the free energy density which is a function of the in-plane angle $\varphi_{\rm m}$ of the magnetization $\mathbf{M} = M_{\rm s}[m_{\rm x}, m_{\rm y}] = M_{\rm s}[\cos(\varphi_{\rm m}), \sin(\varphi_{\rm m})]$. Furthermore, $K_{\rm c1}$ is the cubic anisotropy constant and the external magnetic field is written as $\mu_0\mathbf{H} = \mu_0 H[\cos(\varphi), \sin(\varphi)]$ with $\mu_0 H = 50\,{\rm mT}$ the magnitude of the applied field and $\varphi$ the well-known orientation of the external magnetic field. In Eq. (S10) we only consider the two-dimensional in-plane magnetized case, where we disregard the shape anisotropy contribution due to the magnetic thin film. In order to model the observed angle dependence, Eq. (S10) is numerically minimized with respect to $\varphi_{\rm m}$ for each external magnetic field angle $\varphi$. For this purpose, we use an anisotropy constant $K_{\rm c1} = -600\,{\rm J/m^3}$, which corresponds to the literature value of YIG at room temperature found in Ref. [S19]. To simulate our angle dependent measurement, we replace the $\cos^2(\varphi)$ fitting function with a simulation of the form

$$V_{\rm ac}(\varphi) = A_{I_{\rm dc}=0}\cos^2(\varphi_{\rm m}(\varphi)) + A_{\rm off}, \tag{S11}$$

where $A_{\rm off} = 115\,{\rm nV}$ is the offset voltage signal that we included to quantitatively model our experimental data. The argument of the $\cos^2$ function in Equation (S11) is extracted from the Stoner-Wohlfarth-model and gives the magnetization angle $\varphi_{\rm m}$ as a function of the external magnetic field angle $\varphi$. Equation (S11) is plotted in Fig. S10 (a) (red solid line) together with the respective data (black data points) and the simple $\cos^2(\varphi)$ fit (blue solid line). The simulation that includes the cubic anisotropy shows a much better agreement with the experimental data than the simple $\cos^2(\varphi)$ fit. This observation can be further solidified by plotting the differences $\Delta V_{\rm ac}$ between the data and the fit (i.e. the residual) as well as the difference between the data and the simulation. This is shown in Fig. S10 (b), which displays the residual of the $\cos^2(\varphi)$ fit to the data as the blue data points, while the difference between the data and the simulation is shown as the red points. The residual of the fit to the data (blue points) shows a finite modulation. This is expected for the appearance of a cubic anisotropy in our data, since this is obviously not included in this simple fit. In contrast, the difference of the simulation and the data (red points), shows a vanishing modulation. Hence, we conclude that our data fits well to our simulation, since the angular dependence of the magnon transport signal can be accurately modeled by introcuding a cubic anisotropy to the simulation with an anisotropy constant that corresponds to the literature value [S19].

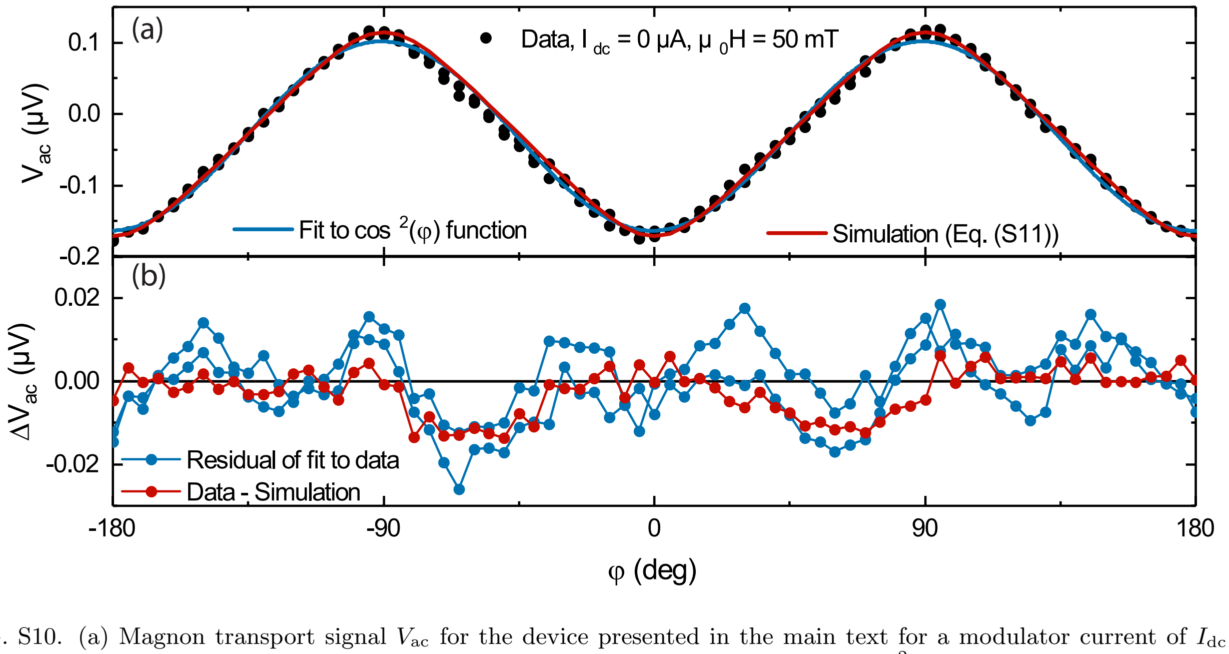


FIG. S10. (a) Magnon transport signal $V_{\rm ac}$ for the device presented in the main text for a modulator current of $I_{\rm dc} = 0\,\mu{\rm A}$ (black data points, see also Fig. 2 in the main text). The blue solid line represents a $\cos^2(\varphi)$-fit to the data, while the red solid line is a simulation based on Eq. (S11). (b) Residual/difference $\Delta V_{\rm ac}$ of the $\cos^2(\varphi)$ fit to the data in (a) (blue points with line) and difference between the simulation and the data (red data points with line).

In the next step, we investigate the impact of the DC current in the modulator on the angle dependent measurements in more detail. The angle dependent measurements shown in Fig. 2 of the main text are altered by the DC current in

the modulator in a threefold manner: (i) via the SHE-induced injection of magnons ($\propto I_{\rm dc}\cos(\varphi)$), (ii) via the thermal injection of magnons ($\propto I_{\rm dc}^2$) and (iii) due to the magnon damping compensation (or BEC/swasing transition), which corresponds to an almost step-like increase of magnon conductivity as a function of $I_{\rm dc}$ (c.f. Fig. 4 (a) in the main text). The deformation of the angular dependent signals due to (i) and (ii) was already reported in Ref. [S2] and allows one to separate the contributions of SHE- and thermally injected magnons by the symmetry of the angular dependence. In order to see whether the SHE- or thermally injected magnons dominate the transition into (iii) (the damping compensated regime), we can expand the model of Ref. [S2] by the step-like increase of magnon conductivity. This is implemented by modelling the magnon conductivity increase due to (iii) by a smooth step function, i.e. a function that is of the form of a Fermi-Dirac distribution. Hence, we can write down the expected angular dependence of the first harmonic detector signal $V_{\rm ac}$ as

$$V_{\rm ac}(\varphi) = A_{\rm I_{dc}=0}\cdot\cos(\varphi)^2\left(\underbrace{1}_{1^{\rm st}\ \rm term} + \underbrace{\frac{\sigma_{\rm m}^{\rm Therm}}{\sigma_{\rm m}^0}I_{\rm dc}^2}_{2^{\rm nd}\ \rm term} + \underbrace{\frac{\sigma_{\rm m}^{\rm SHE}}{\sigma_{\rm m}^0}I_{\rm dc}\cos(\varphi)}_{3^{\rm rd}\ \rm term} + \underbrace{\frac{\sigma_{\rm m}^{\rm crit}}{\sigma_{\rm m}^0}\left(1-\frac{1}{\exp\left(\frac{I_{\rm dc}\cos(\varphi)-I_{\rm trans}}{\Delta I}\right)+1}\right)}_{4^{\rm th}\ \rm term\equiv L_{crit}^{SHE}}\right) + A_{\rm off}. \tag{S12}$$

Equation (S12) consists of four terms: the first term corresponds to the undisturbed magnon transport between injector and detector and scales with the magnon conductivity $\sigma_{\rm m}^0$ of YIG. The second term describes the quadratic scaling of the magnon conductivity modulation $\sigma_{\rm m}^{\rm Therm}$ due to the thermal injection of magnons by the heating of the DC current. The SHE-induced magnon conductivity enhancement $\sigma_{\rm m}^{\rm SHE}$ in the third term scales linearly with $I_{\rm dc}$ and is modulated with a $\cos(\varphi)$ function. Finally, the fourth term, which we call $L_{\rm crit}^{\rm SHE}$, represents the critical magnon conductivity enhancement $\sigma_{\rm m}^{\rm crit}$ due to the damping compensation, which is multiplied by a Fermi-Dirac-like function. Here, $I_{\rm trans}$ corresponds to the DC current where the magnon conductivity is increased by half of $\sigma_{\rm m}^{\rm crit}$ (i.e. $I_{\rm trans}\approx\frac{I_{\rm on}+I_{\rm crit}}{2}\approx 0.5\,\rm mA$) and $\Delta I\approx\frac{I_{\rm crit}-I_{\rm on}}{2}\approx 50\,\rm\mu A$ gives the smearing of the step function. In this model, we assume that the critical behaviour observed in our experiments stems from the SHE-induced magnons. This is included in the model since the DC current $I_{\rm dc}$ in the exponential function of Eq. (S12) is multiplied by a $\cos(\varphi)$ function, which accounts for the effective magnitude of $I_{\rm dc}$ that is injecting magnons into the YIG via the SHE (i.e. the projection of the spin polarization of the SHE-inudced spin chemical potential $\mu_{\rm s}$ on the direction perpendicular to the Pt electrodes). In contrast, assuming that the thermal injection of magnons dominates the critical behaviour described by $L_{\rm crit}^{\rm SHE}$ in Eq. (S12), no additional angle dependence should appear in this term.

To check the validity of the model presented in Eq. (S12), we first calculate each of the conductivity contributions (i.e. $\sigma_{\rm m}^{\rm SHE}$, $\sigma_{\rm m}^{\rm Therm}$ and $\sigma_{\rm m}^{\rm crit}$) for an external magnetic field of $\mu_0 H = 50\,\rm mT$. For this purpose, we use Eq. (S8) to calculate the YIG spin resistance changes $\Delta R^{\rm s}_{\rm YIG,SHE/Therm}$. We extract the changes in the signal amplitude $A_{\rm SHE}$ ($A_{\rm Therm}$) due to the SHE-induced injection (thermal injection) of magnons by fitting a linear (quadratic) function to the respective linear (quadratic) regime in Fig. S5 (a) ((b)). The slope $\frac{{\rm d}\eta_{\rm SHE}}{{\rm d}I_{\rm dc}}$ and the second order coefficient $\frac{{\rm d}^2\eta_{\rm Therm}}{{\rm d}I_{\rm dc}^2}$ of these fits, respectively, are multiplied by $A_{\rm I_{dc}=0}$, by which we get $\frac{{\rm d}A_{\rm SHE}}{{\rm d}I_{\rm dc}} = 173.93\,\rm\mu V/A$ and $\frac{{\rm d}^2A_{\rm Therm}}{{\rm d}I_{\rm dc}^2} = 315.38\,\rm mV/A^2$[S20]. These values are substituted for the voltage amplitudes in Eq. (S9), from which we calculate the resistance changes via Eq. S8. Finally, we use [S16]

$$\sigma_{\rm m}^{\rm SHE/Therm} = \frac{d}{\Delta R^{\rm s}_{\rm YIG,SHE/Therm}A_{\rm YIG}} \tag{S13}$$

to calculate the respective conductivity modulations (in units of $(1/(\Omega\rm mA)$ for $\sigma_{\rm m}^{\rm SHE}$ and $1/(\Omega\rm mA^2)$ for $\sigma_{\rm m}^{\rm Therm}$). Here, $A_{\rm YIG} = t_{\rm YIG}l_{\rm Pt}$ is the cross section of the YIG transport channel and $d = 1.3\,\rm\mu m$ is the edge-to-edge distance between injector and detector. We find $\sigma_{\rm m}^{\rm SHE} = 1.2\times10^6\,1/(\Omega\rm mA)$ and $\sigma_{\rm m}^{\rm Therm} = 2.2\times10^{12}\,1/(\Omega\rm mA^2)$. To calculate $\sigma_{\rm m}^{\rm crit}$, we estimate the resistance in the uncompensated regime (for $I_{\rm dc} < I_{\rm on}$) and in the compensated regime (for $I_{\rm dc} > I_{\rm crit}$) from Fig. 4 (a) of the main text and find $R^{\rm s}_{\rm YIG,on}\approx 0.31\,\Omega$ and $R^{\rm s}_{\rm YIG,crit}\approx 0.18\,\Omega$, respectively. Subsequently, we calculate the magnon conductivity change due to to the damping compensation as $\sigma_{\rm m}^{\rm crit} = \frac{d}{A_{\rm YIG}}(1/R^{\rm s}_{\rm YIG,crit} - 1/R^{\rm s}_{\rm YIG,on}) = 1.4\times10^6\,1/(\Omega\rm m)$. With these values, we can simulate the angular dependence for different DC currents $I_{\rm dc}$ via Eq. (S12). The result is shown in Fig. S11 (a) for three different DC currents (filled circles in black, green and orange). To get a more acccurate simulation of our data, we also included the cubic anisotropy contribution to the angle dependence in Eq. (S12) via the Stoner-Wohlfarth model presented in Eq. S10. Since the cubic anisotropy constant $K_{\rm c1}$ decreases with increasing temperature in YIG [S19] and the large heating effect of the modulator

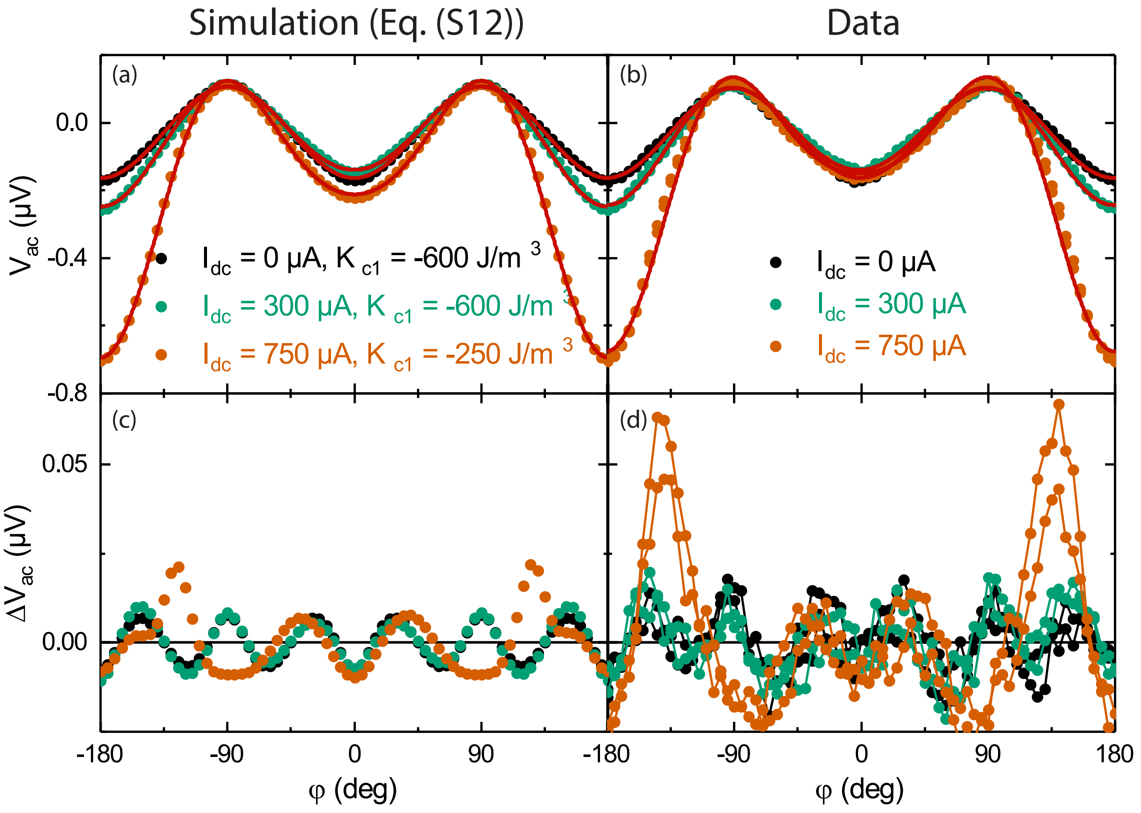


FIG. S11. (a) Simulated angular dependence of the first harmonic detector signal $V_{\rm ac}$ via Eq. (S12) for different DC currents $I_{\rm dc}$ and an external magnetic field $\mu_0 H = 50\,\rm mT$ (filled circles). The red solid lines are fits to Eq. (S14). (b) Experimental data of the first harmonic detector signal as a function of $\varphi$ (c.f. Fig. 2 of the main text). Solid red lines are again fits to Eq. (S14). (c) Residuals of the fits to the simulated angular dependence. (d) Residuals of the fits to the experimental data.

current increases the local sample temperature up to $\sim 370\,\rm K$ (see thermometry measurements in Sec. IV), we chose a corresponding smaller anisotropy constant of $K_{\rm c1} = -250\,\rm J/m^3$ for the largest DC current of $I_{\rm dc} = 750\,\mu\rm A$. In order to compare the model to our data, Fig. S11 (b) shows the corresponding angle dependent experimental results of the device presented in the main text (c.f. Fig. 2 in the main text). The simulation in panel (a) shows a decent quantitative agreement with the experimental data in panel (b) for the calculated magon conductivity contributions (i.e. $\sigma_{\rm m}^{\rm SHE}$, $\sigma_{\rm m}^{\rm Therm}$ and $\sigma_{\rm m}^{\rm crit}$). To see if our simulation actually models the observed angular dependence accurately, we fit both the experimental data as well as the simulations with a function of the form

$$V_{\rm ac}(\varphi) = C\cos(\varphi)^2 + D\cos(\varphi)^3 + E. \tag{S14}$$

These fits are shown in Fig. S11 (a) and (b) by the red solid lines. Comparing our fitting function in Eq. (S14) to the model in Eq. (S12), we can identify the fit parameters as $C = A_{\rm I_{dc}=0}(1 + \frac{\sigma_{\rm m}^{\rm Therm}}{\sigma_{\rm m}^0} I_{\rm dc}^2)$, $D = A_{\rm I_{dc}=0}\frac{\sigma_{\rm m}^{\rm SHE}}{\sigma_{\rm m}^0} I_{\rm dc}$ and $E = A_{\rm off}$. Hence, $C$ corresponds to the first and second term in Eq. (S12), while parameter $D$ is proportional to the third term. The fourth term $L_{\rm crit}^{\rm SHE}$, however, contains another angle dependence, which is not included in Eq. (S14). This is because the $\cos(\varphi)$ term appears in the exponential function in this term and is therefore not included in any of the fitting parameters used. Thus, this specific angular dependence should appear as the residual of the fit. Moreover, since the cubic anisotropy is not included in the fit of Eq. (S14) either, we expect this to appear in the residuals as well. We therefore plot the residual $\Delta V_{\rm ac}$ of the fit to the simulation and the residual of the fit to the experimental data in Fig. S11 (c) and (d), respectively. For $I_{\rm dc} < I_{\rm trans}$ (black and green circles), the residuals of both the simulation (panel (c)) and the experimental data (panel (d)) display the 6-fold angular symmetry that we already observed in the residual shown in Fig. S10 (b). However, there is no indication of a further different angle dependence stemming from the $L_{\rm crit}^{\rm SHE}$ in Eq. (S12). This is expected, since $L_{\rm crit}^{\rm SHE}$ should not have an influence for $I_{\rm dc} < I_{\rm trans}$, where there is no effect of the step-like magnon conductivity increase. For $I_{\rm dc} = 750\,\mu\rm A > I_{\rm trans}$, however, the residuals of both the simulation and the experimental data change their symmetry to a more complex structure (orange circles

in panels (c) and (d)). Most importantly, the angular symmetries of both the simulated and experimental residuals qualitatively agree with each other. However, a full quantitative agreement with this simple phenomenlogical model could not be achieved and thus a deeper theoretical understanding of the relevant processes is needed to fully explain the observed experimental data.Hence, we conclude that the model presented in Eq. (S12) (where the SHE-induced magnon injection is assumed to be responsible for the damping compensation) is valid and supports our claim that the SHE is the dominant contribution to the threshold behaviour observed in our experiments.

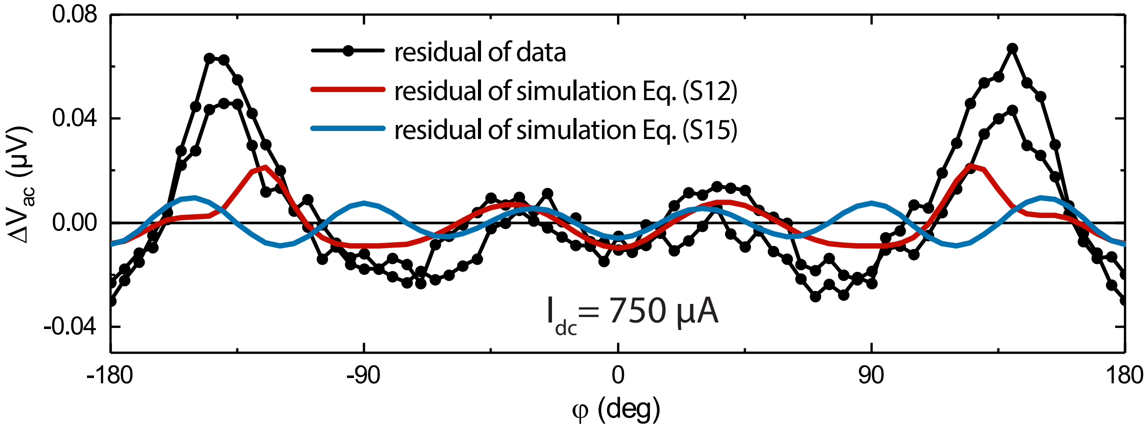


FIG. S12. Residual of the fit (Eq. (S14)) to the experimental data of Fig. S11 for $I_{\mathrm{dc}} = 750\,\mu\mathrm{A}$ (black data points). The solid red line shows the residual of the fit to the simulated angular dependency based on Eq. (S12) (see Fig. S11 (c)). The solid blue line represents the residual of the fit to the simulated angular dependence when thermal magnons are assumed to be responsible for the damping compensation (i.e. when $L_{\mathrm{crit}}^{\mathrm{SHE}}$ in Eq. (S12) is replaced by Eq. (S15)).

As a next step, we can check the validity of our model by changing Eq. (S12) in a way that we no longer assume the SHE-induced magnons to be responsible for the damping compensation (or BEC/swasing transition), but rather the thermally injected magnons. This can be done by omitting the cos($\varphi$) function in $L_{\mathrm{crit}}^{\mathrm{SHE}}$ of Eq. (S12), leading to

$$L_{\mathrm{crit}}^{\mathrm{Therm}} = \frac{\sigma_{\mathrm{m}}^{\mathrm{crit}}}{\sigma_{\mathrm{m}}^{0}} \left(1 - \frac{1}{\exp\left(\frac{I_{\mathrm{dc}} - I_{\mathrm{trans}}}{\Delta I}\right) + 1}\right). \tag{S15}$$

In this way, we assume that there is no magnetization orientation dependency regarding the critical behaviour described by Eq. S15, which should be the case if the thermal injection of magnons dominates the observed critical enhancement of the magnon conductivity. We replace $L_{\mathrm{crit}}^{\mathrm{SHE}}$ in Eq. (S12) by $L_{\mathrm{crit}}^{\mathrm{Therm}}$ described by Eq. (S15) and fit the resulting model with Eq. (S14) for a DC current of $I_{\mathrm{dc}} = 750\,\mu\mathrm{A} > I_{\mathrm{trans}}$. The residual of the fit to this altered model is shown in Fig. S12 as the blue solid line. We immediately see that the angular symmetry is now equal to the 6-fold symmetry stemming from the cubic anisotropy (see Fig. S10). This is expected, since the critical behaviour described by Eq. (S15) does not include an additional angle symmetry and is therefore fully contained in the fit parameter $C$ in Eq. (S14). For comparison, we again plot the residual of the simulation based on Eq. (S12) (which assumes the SHE induced magnons to be responsible for the critical behaviour, see Fig. S11 (c)) as the red solid line in Fig. S12. Additionally, the experimentally extracted residual shown in Fig. S11 (d) is shown in Fig. S12 for $I_{\mathrm{dc}} = 750\,\mu\mathrm{A}$ as well (black data points with line). Here, we find that both the simulation based on Eq. (S12) (red solid line) as well as the experimentally extracted residual (black data points) qualitatively match (as already observed in Fig. S11 (c) and (d)). The quantitative agreement on the other hand is rather poor. This, however, is not very surprising, since the exact dependence of the angle dependent measurements is strongly affected by the exact form of the step-like increase of magnon conductivity. The Fermi-Dirac-like function in our model does only crudely reproduce the observed $I_{\mathrm{dc}}$-dependence of the magnon conductivity. This is also the reason why the peak position of the simulated residuals at $\varphi \approx -125°$ and $\varphi \approx 125°$ do not properly coincide with the experimentally observed positions at $\varphi \approx -140°$ and $\varphi \approx 140°$.

In conclusion, we can only achieve an accurate phenomenological modelling of the experimentally observed angle dependence, when we assume the SHE-induced magnons to dominate the critical behaviour described by $L_{\mathrm{crit}}^{\mathrm{SHE}}$ in Eq. (S12). When thermal magnons are assumed to be responsible for the critical behaviour, which can be modelled by replacing $L_{\mathrm{crit}}^{\mathrm{SHE}}$ in Eq. (S12) by $L_{\mathrm{crit}}^{\mathrm{Therm}}$ (Eq. (S15)), we do not find a proper agreement of our data with the model (see Fig. S12). We therefore conclude that indeed the electrically injected magnons via the SHE are the dominant

contribution to the damping compensation (or BEC/swasing transition) in our experiment. We want to emphasize, that our modelling does not prove that the thermal injection of magnons cannot be responsible for the damping compensation in general. In order to investigate this in more detail, one could think of employing our experiment by replacing the modulator with a light metal. Alternatively, one could insert an insulating layer in between the Pt modulator electrode and the YIG surface. In both cases, one could switch off the SHE-induced injection of magnons and therefore study the thermal magnon conductivity modulation separately. We do, however, not believe that such a damping compensation can be achieved by a thermal injection of magnons alone. This is because previous theoretical considerations suggest that any finite temperature difference at the Pt/YIG interface always leads to an increase of the threshold condition for damping compensation [S9].

## IX. SECOND HARMONIC MAGNON TRANSPORT SIGNALS

The second harmonic signal at the detector is sensitive to the thermally injected magnons from the injector. Since the diffusive transport of magnons in YIG was shown to be dominated by the magnon chemical potential profile for both electrically as well as thermally injected magnons [S16], we expect the same signatures in the second harmonic signals. It is important to note that a finite temperature difference at the detector electrode, induced by the heating in the injector, does indeed also lead to a local spin Seebeck effect in the detector. However, it was shown that this 'local' effect does only play a major role for distances between the electrodes that are approximately smaller than the YIG thickness [S21]. In our case, where we use a very thin YIG film with a 13.4 nm thickness, we assume thermal effects in the detector to be dominated by the chemical potential driven magnon transport. In Fig. S13 (a) and (b) we plot the angle dependent second harmonic magnon transport signal $V_{2\omega}$ for both positive and negative DC current biases, respectively. As expected, we find a significant enhancement of the magnon transport signal for the same magnetic field orientations as observed for the first harmonic signals in the main text.

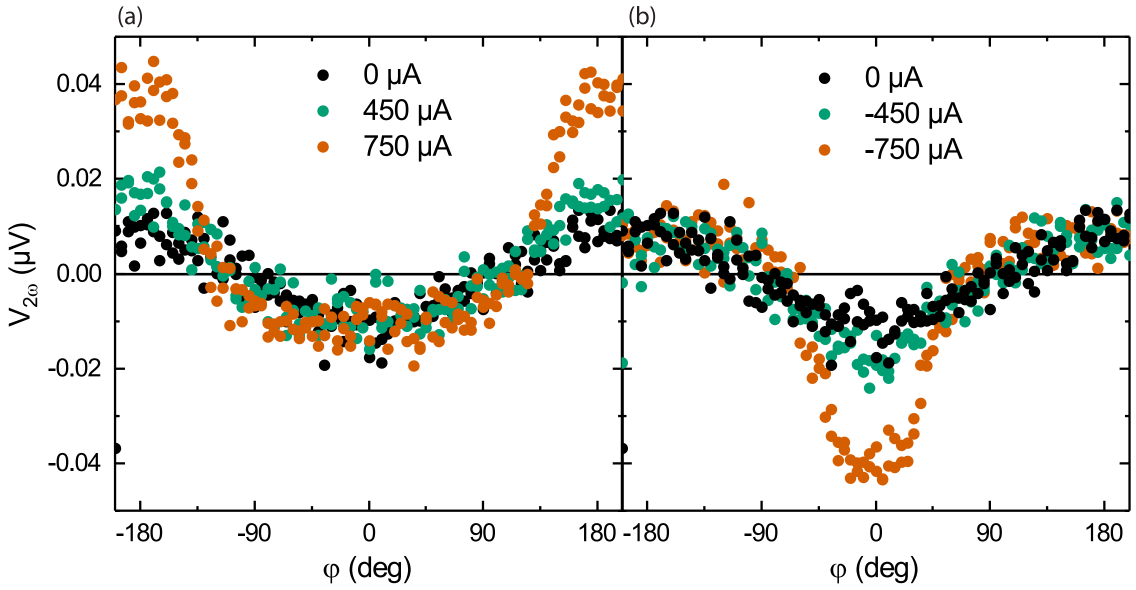


FIG. S13. Magnetic field orientation dependent second harmonic signal $V_{2\omega}$ at the detector for (a) positive and (b) negative DC currents in the modulator for an external magnetic field of $\mu_0 H = 50\,\mathrm{mT}$.

Subsequently, we directly compare the first and second harmonic signals at the detector as a function of the applied modulator current $I_{\mathrm{dc}}$. We therefore plot the respective I-V-characteristics of the first and second harmonic voltage signals $V_{1\omega}$ and $V_{2\omega}$ in Fig. S14 (a) and (c) for both positive and negative field orientations, respectively. Similar to the first harmonic signals discussed in the main text, we find a very significant kink in the I-V-characteristics for $V_{2\omega}$. In order to compare the two contributions in more detail, we correct both signals for the SHE-induced (linear in $I_{\mathrm{dc}}$) and thermal (quadratic in $I_{\mathrm{dc}}$) modulation effects of the magnon conductivity. This correction is done as described in Section VI and shown in Fig. S14 (b) and (d). For both signals, we find a constant regime for small currents $I_{\mathrm{dc}} < 0.4\,\mathrm{mA}$ and a steep increase in the measured voltage signals for larger currents. While $V_{1\omega}^{\mathrm{corr}}$ seems to saturate beyond the critical current $I_{\mathrm{crit}}$, the second harmonic $V_{2\omega}^{\mathrm{corr}}$ increases further and seems to saturate for larger currents

as compared to $V_{1\omega}^{\mathrm{corr}}$. Moreover, the onset current $I_{\mathrm{on}}$ observed for the first harmonic does not perfectly match with the onset of the magnon conductivity increase in the second harmonic. A more rigorous analysis of the second harmonic signals in our experiment might be beneficial regarding the magnon BEC interpretation of our results. This is due to the fact, that theoretical considerations on the magnon BEC phase in normal metal/magnetic insulator heterostructures suggest, that the spin Seebeck effect should decrease when entering the BEC phase [S22]. Since the thermal conductivity, similar to a conventional superfluid, becomes very large in the magnon BEC phase [S22], the spin Seebeck effect at the interface of such structure is expected to decrease. Signatures of this effect might be possible to measure by the second harmonic signal within the framework of our magnon conductivity measurement. Due to the rather low injection current of $I_{\mathrm{ac}} = 50\,\mu\mathrm{A}$, however, the thermal signals are relatively small and a rigorous analysis of the data is tedious. Furthermore, even larger currents might be necessary to see this effect in our data. We therefore concentrate on the first harmonic signals in the main text. In general, the qualitative signatures of the first and second harmonic signals are very similar, but the quantitative details seem to differ. We therefore conclude that both electrically as well as thermally driven magnon transport is in principle suitable to observe the critical magnon conductivity enhancement in our experiments.

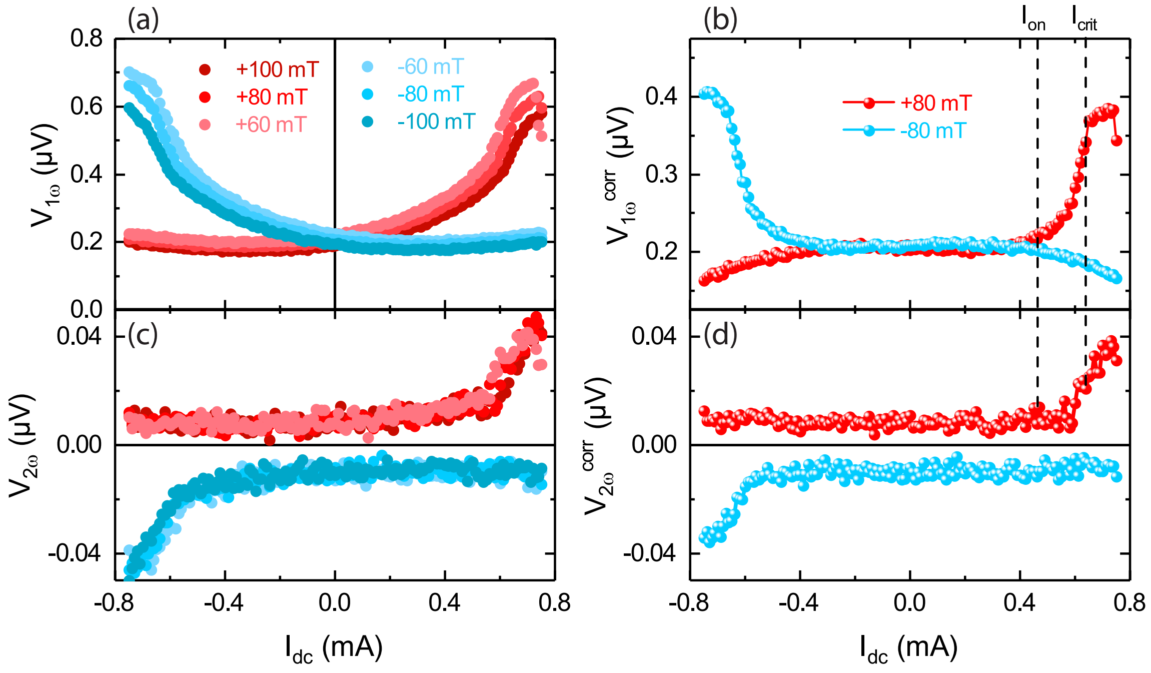


FIG. S14. (a) First harmonic voltage signals $V_{1\omega}$ as a function of $I_{\mathrm{dc}}$ for both positive (red data points) and negative (blue data points) external fields. Red data points correspond to the field direction along $\varphi = \pm 180°$, while blue data points correspond to $\varphi = 0°$. (b) Corrected first harmonic signal $V_{1\omega}^{\mathrm{corr}}$, where SHE-induced (linear) and thermal (quadratic) modulation of the magnon transport is subtracted (see Section VI and Eq. (S7)). (c) Second harmonic signal $V_{2\omega}$ versus $I_{\mathrm{dc}}$ analogous to panel (a). (d) Corrected second harmonic signal $V_{1\omega}^{\mathrm{corr}}$ analogous to panel (b).

## X. COMPARISON BETWEEN SPIN HALL NANO-OSCILLATORS AND DC PUMPED MAGNON BEC

In this Section, we want to discuss the strong correlation between the theories of spin Hall nano-oscillators (SHNOs) [S23, S24] and the DC pumped magnon BEC put forward in Ref. S9 for the YIG/Pt bilayer investigated in this work. In general, both concepts basically describe a coherent oscillation of magnetization that is dynamically sustained via spin-orbit torques. While spin Hall auto-oscillations are described within a fully classical Landau-Lifshitz-Gilbert (LLG) model, the DC pumped magnon BEC theory relies on a quantum mechanical description of the magnons in the condensate.

We start with the well-established description of SHNOs. Here, auto-oscillation of the magnetization is achieved when the spin torque generated via the SHE compensates the intrinsic damping of the magnetic layer. The damping rate is given by

$$\Gamma_{\mathrm{D}}^{\mathrm{oop}} = (\alpha_{\mathrm{G}} + \alpha_{\mathrm{sp}})\,\gamma\mu_0\,(H - M_{\mathrm{s}}) \tag{S16}$$

for an out-of-plane magnetized film and by

$$\Gamma_{\mathrm{D}}^{\mathrm{ip}} = (\alpha_{\mathrm{G}} + \alpha_{\mathrm{sp}})\,\gamma\mu_0\left(H + \frac{M_{\mathrm{s}}}{2}\right) \tag{S17}$$

for an in-plane magnetized film [S25, S26]. Here, $\alpha_{\mathrm{G}}$ is the Gilbert damping, $\alpha_{\mathrm{sp}}$ the spin pumping induced damping, $\gamma$ the gyromagnetic ratio, $H$ the external field and $M_{\mathrm{s}}$ the saturation magnetization. Note, that Eq. (S16) and Eq. (S17) simply correspond to the FMR linewidth $\Delta\omega = (\alpha_{\mathrm{G}} + \alpha_{\mathrm{sp}})\mu_0\gamma\left(H + \frac{M_{\mathrm{s}}}{2}(N_{\mathrm{x}} + N_{\mathrm{y}} - 2N_{\mathrm{z}})\right)$ for thin films in the presence of spin-pumping induced damping $\alpha_{\mathrm{sp}}$ (with demagnetization factors $N_{\mathrm{i}}$, where $N_{\mathrm{x}} = N_{\mathrm{z}} = 0$, $N_{\mathrm{y}} = 1$ for in-plane and $N_{\mathrm{x}} = N_{\mathrm{y}} = 0$, $N_{\mathrm{z}} = 1$ for out-of-plane). The anti-damping spin torque rate due to the SHE in the macrospin approximation is given by [S24]

$$\Gamma_{\mathrm{ST}} = \frac{\hbar}{2e}\frac{\gamma}{M_{\mathrm{s}}t_{\mathrm{YIG}}t_{\mathrm{Pt}}w}\cdot T\cdot\theta_{\mathrm{SH}}I_{\mathrm{dc}} \tag{S18}$$

with $t_{\mathrm{YIG}}$ the film thickness of the YIG layer, $\theta_{\mathrm{SH}}$ the spin Hall angle of the Pt and $I_{\mathrm{dc}}$ the DC current applied to the Pt strip with thickness $t_{\mathrm{Pt}}$ and width $w$. $T$ denotes the interface transparency for spin currents as put forward in Ref. S4 and reads as

$$T = \frac{g^{\uparrow\downarrow}\tanh(\eta)}{g^{\uparrow\downarrow} + \frac{\hbar}{2e^2}\frac{\sigma_{\mathrm{e}}}{l_{\mathrm{s}}}}, \tag{S19}$$

where $\eta = \frac{t_{\mathrm{Pt}}}{2l_{\mathrm{s}}}$ with the spin diffusion length $l_{\mathrm{s}}$ of Pt and the thickness $t_{\mathrm{Pt}}$ of the Pt strip. We approximated $\coth(2\eta) \approx 1$ in Eq. (S19). When the condition $\Gamma_{\mathrm{D}}^{\mathrm{ip}} = \Gamma_{\mathrm{ST}}$ is met, a coherent precession of the magnetization with zero effective damping is present [S25].

In the DC pumped magnon BEC theory put forward in Ref. S9, Bender et al. give two threshold conditions for either the magnon BEC transition and the swasing transition. For the spin chemical potential at the YIG/Pt interface (for an out-of-plane magnetized film), these criteria read as

$$\mu_{\mathrm{c=2/c=1}}^{\mathrm{oop}} = \left(1 + \frac{\alpha_{\mathrm{G}}}{c\cdot\alpha_{\mathrm{sp}}}\right)\hbar\Omega \tag{S20}$$

Here, $\Omega = \gamma\mu_0(H - M_{\mathrm{s}})$ denotes the fundamental ferromagnetic resonance frequency for an out-of-plane magnetized film. Note, that the ratio $\frac{\alpha_{\mathrm{G}}}{\alpha_{\mathrm{sp}}}$ in Eq. (S20) accounts for the interface spin transparency in this model. As explained in the main text, the parameter $c$ distinguishes between the magnon BEC transition $\mu_{\mathrm{c=2}}^{\mathrm{oop}}$ and the swasing transition $\mu_{\mathrm{c=1}}^{\mathrm{oop}}$. For the swasing threshold with $c = 1$, we find

$$\mu_{\mathrm{c=1}}^{\mathrm{oop}} = \frac{\hbar}{\alpha_{\mathrm{sp}}}\Gamma_{\mathrm{D}}^{\mathrm{oop}}. \tag{S21}$$

The direct proportionality of $\mu_{\mathrm{c=2/c=1}}^{\mathrm{oop}}$ to the FMR frequency $\Omega$ is solely valid for an out-of-plane magnetized film. For the in-plane configuration, we instead have to consider the in-plane frequency linewidth and obtain

$$\mu_{\mathrm{c=1}}^{\mathrm{ip}} = \frac{\hbar}{\alpha_{\mathrm{sp}}}\Gamma_{\mathrm{D}}^{\mathrm{ip}} = \left(1 + \frac{\alpha_{\mathrm{G}}}{\alpha_{\mathrm{sp}}}\right)\hbar\gamma\mu_0\left(H + \frac{M_{\mathrm{s}}}{2}\right), \tag{S22a}$$

$$\mu_{\mathrm{c=2}}^{\mathrm{ip}} = \left(1 + \frac{\alpha_{\mathrm{G}}}{2\alpha_{\mathrm{sp}}}\right)\hbar\gamma\mu_0\left(H + \frac{M_{\mathrm{s}}}{2}\right). \tag{S22b}$$

The spin chemical potential at the YIG/Pt interface induced via the SHE reads [S16, S27, S28]

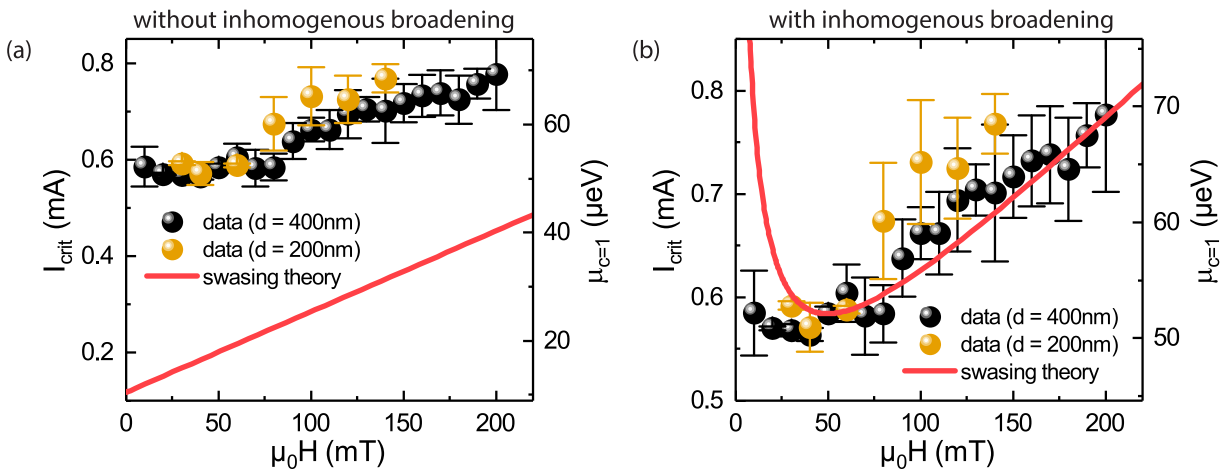


FIG. S15. Critical current $I_{\text{crit}}$ plotted versus the externally applied magnetic field $\mu_0 H$. Panel (a) shows the theory curve (red line) without considering inhomogenous broadening, while panel (b) includes inhomogenous broadening via the effective damping parameter $\alpha_{\text{eff}}$. Both panels include the experimental data presented in the main text and additional data for a device with an edge-to-edge strip separation of $d = 200\,\text{nm}$.

$$\mu_{\text{s}} = \frac{e\theta_{\text{SH}} I_{\text{dc}}}{w\sigma_{\text{e}}\eta} \tanh{(\eta)} \tag{S23}$$

We now combine Eq. (S4), (S17), (S18) and (S19) and find $\mu_{\text{s}} = \frac{\hbar}{\alpha_{\text{sp}}}\Gamma_{\text{ST}}$. Hence the swasing threshold $\mu_{\text{s}} = \mu_{\text{c}=1}$ is indeed fully identical to the SHNO threshold $\Gamma_{\text{ST}} = \Gamma_{\text{D}}$ for in-plane and out-of plane configurations.

We can now solve the critical conditions for the DC current $I_{\text{dc}}$ by equating Eqs. (S22a) ((S22b)) and (S23). Using Eq. (S3), we find the critical currents

$$I_{\text{on}} = \frac{\eta w \sigma_{\text{e}}}{e\theta_{\text{SH}}} \coth{(\eta)} \left(1 + 2\pi M_{\text{s}} t_{\text{YIG}} \frac{\alpha_{\text{G}}}{\hbar\gamma g_{\text{eff}}}\right) \hbar\gamma\mu_0 \left(H + \frac{M_{\text{s}}}{2}\right), \tag{S24a}$$

$$I_{\text{crit}} = \frac{\eta w \sigma_{\text{e}}}{e\theta_{\text{SH}}} \coth{(\eta)} \left(1 + 4\pi M_{\text{s}} t_{\text{YIG}} \frac{\alpha_{\text{G}}}{\hbar\gamma g_{\text{eff}}}\right) \hbar\gamma\mu_0 \left(H + \frac{M_{\text{s}}}{2}\right). \tag{S24b}$$

In Fig. S15 (a), the swasing threshold current $I_{\text{crit}}$ is plotted as a function of the external magnetic field $\mu_0 H$ (red line). Additionally, we included the experimental data presented in the main text with additional data of a device with an edge-to-edge strip separation of $d = 200\,\text{nm}$. Obviously, the theoretical model does not yet quantitatively describe the experimental data well. This is due to the fact that the inhomogeneous broadening has to be considered, as demonstrated in Ref. S24. To this end, we follow Ref. S24 and introduce an effective (frequency-dependent) damping parameter

$$\alpha_{\text{eff}} = \alpha_{\text{G}} + \gamma\mu_0 \frac{\delta H}{2\omega_{\text{FMR}}^{\text{ip}}} \tag{S25}$$

where the second term accounts for the damping introduced via the inhomogenous broadening $\delta H$ of the magnetic thin film. The FMR frequency $\omega_{\text{FMR}}^{\text{ip}} = \gamma\mu_0\sqrt{H(H + M_{\text{s}})}$ is calculated from the Kittel formula for the in-plane configuration. By substituting $\alpha_{\text{G}}$ with $\alpha_{\text{eff}}$ in Eq. S24, we find the theory curves plotted in Fig. S15 (b) and Fig. 4b in the main text. Note, that the strong increase of the theory curve for small magnetic fields is due to the frequency dependent second term in Eq. S25. Hence, the effective damping $\alpha_{\text{eff}}$ diverges when the magnetic field approaches zero. The slight discrepancy between experimental data and theory for $\mu_0 H < 50\,\text{mT}$ in Fig. S15 (b) might stem from the in-plane magnetocrystalline anisotropy (see Sec. VIII), which could be included by substituting $H \to H + H_{\text{ani}}$ in Eqs. (S24) and (S25) (where $H_{\text{ani}}$ denotes the anisotropy field). Additionally, also the Oersted field generated by the modulator current might change the effective field that is present. This would lead to an effective shift of the experimental data in Fig. S15 (b) along the magnetic field axes. The values used for the model can be found in

| | Symbol | Value | Unit |
|---|---|---|---|
| Pt strip thickness | $t_{\mathrm{Pt}}$ | 3.5 | nm |
| Pt strip width | $w$ | 500 | nm |
| Pt spin diffusion length [S30] | $l_{\mathrm{s}}$ | 1.5 | nm |
| Pt spin Hall angle [S30] | $\theta_{\mathrm{SH}}$ | 0.11 | |
| Pt conductivity | $\sigma_{\mathrm{e}}$ | $1.74 \times 10^{6}$ | $1/\Omega\mathrm{m}$ |
| YIG thickness | $t_{\mathrm{YIG}}$ | 13.4 | nm |
| gyromagnetic ratio | $\gamma$ | $1.78 \times 10^{11}$ | rad/Ts |
| YIG saturation magnetization | $\mu_0 M_{\mathrm{s}}$ | 140 | mT |
| spin mixing conductance | $g^{\uparrow\downarrow}$ | $1.55 \times 10^{19}$ | $1/\mathrm{m}^2$ |
| effective spin mixing conductance | $g_{\mathrm{eff}}$ | $7.6 \times 10^{18}$ | $1/\mathrm{m}^2$ |
| Gilbert damping | $\alpha_{\mathrm{G}}$ | $2.17 \times 10^{-3}$ | |
| spin pumping induced damping | $\alpha_{\mathrm{sp}}$ | $6.0 \times 10^{-3}$ | |
| inhomogenous broadening | $\mu_0 \delta H$ | 3.6 | mT |

TABLE S2. Values for the parameters of Eq. (S22) and (S23) used for the theory curves in Fig. S15.

Tab. S2. In order to get the quantitative agreement with the experimental data, we used an inhomogenous broadening of $\mu_0\delta H = 3.6\,\mathrm{mT}$. In Sec. II we found an experimentally determined value of $\mu_0\delta H = 2.54\,\mathrm{mT}$ for the 24.5 nm thick YIG film investigated for the FMR experiments. It is reasonable to assume that the thinner YIG film (13.4 nm) used for the experiments described in the main text has a slightly larger inhomogeneous broadening. Note, that the (effective) spin mixing conductance in our system is mostly responsible for the temperature dependence of the threshold current(s) in Eqs. S24. As experimentally and theoretically shown, the spin transfer at the YIG/Pt interface decreases when decreasing the temperature [S16, S29]. Intuitively, this temperature dependence is due to the fact that the SHE-induced spin injection at the YIG/Pt interface is related to the coupling to the thermal magnon gas in the YIG. Therefore, magnons can only be excited when a finite number of thermal magnons is present in the YIG [S16, S29]. Hence, the spin transfer basically scales with the number of thermally excited magnons. At lower temperature, the threshold current is therefore expected to increase.

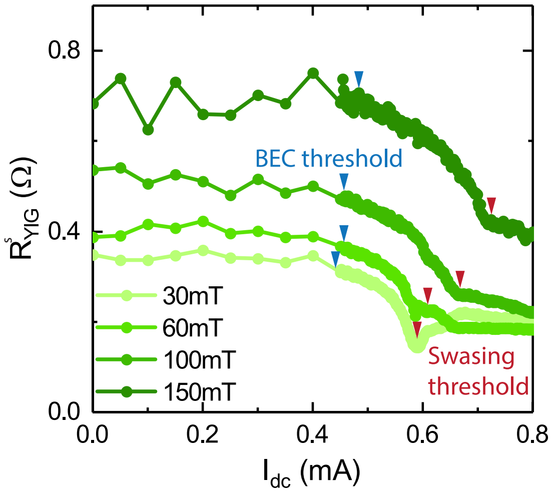


FIG. S16. YIG spin resistance for different magnetic fields. We define the magnon BEC threshold as the current, at which the spin resistance drops by 10 % compared to the constant spin resistance for $I_{\mathrm{dc}} < 0.3\,\mathrm{mA}$ (blue triangles). In the spin resistance picture, the swasing threshold is defined by the onset of the low resistance state (red triangles).

As a last note in this Section, we plot $R^{\mathrm{s}}_{\mathrm{YIG}}$ as a function of DC current for different magnetic fields in Fig. S16 (a). Here, we indicated the critical swasing currents by red triangles and the critical magnon BEC currents by blue triangels. As mentioned in the main text, we find good agreement between the theoretically expected and experimentally determined BEC phase transition. While the data in Fig. 4b in the main text does not provide a final experimental verification of the model in Ref. S9, we conclude that the identification of two distinct threshold conditions for a magnon BEC (with characteristic currents $I_{\mathrm{on}}$ and $I_{\mathrm{crit}}$) is justified.

## XI. IMPACT OF COHERENT MICROWAVE DRIVEN MAGNETIZATION PRECESSION ON MAGNON CONDUCTIVITY MEASUREMENTS

In the previous Section, we found that the physics of spin torque oscillators and the swasing phase of a DC pumped magnon BEC are identical, since both theories describe a coherent oscillation of the magnetization precession due to a compensation of the magnetic damping. In our experiment, we found that the magnon conductivity is very strongly enhanced when the magnons are transported through the damping compensated region. Since this might be an indicator for a the generation of a coherent magnetization precession (i.e. magnon BEC or swasing), we now test whether the magnon transport is also affected by coherent precession of the magnetization due to ferromagnetic resonance. Similar experiments have been recently put forward by Liu et al. in Ref. S31.

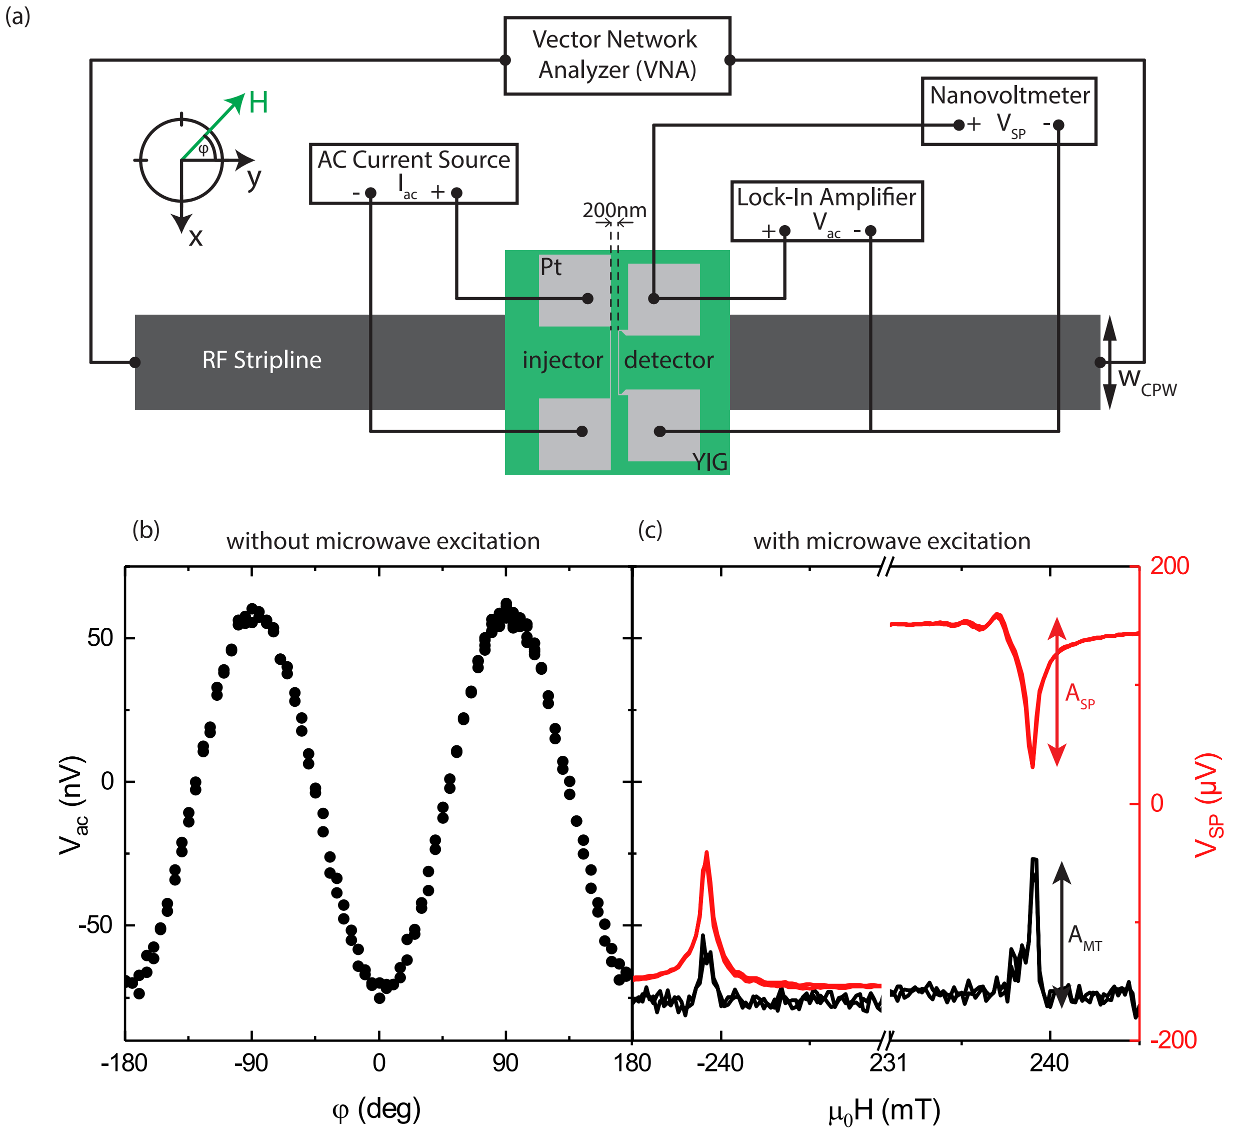


FIG. S17. (a) Schematic illustration of the experimental setup. The sample is placed onto a CPW with a width of $w_{\mathrm{CPW}} = 1\,\mathrm{mm}$, which is connected to a VNA acting as the microwave source and detector. The injector strip is sourced with a low frequency ($f = 13\,\mathrm{Hz}$) AC current $I_{\mathrm{ac}} = 100\,\mu\mathrm{A}$, while the magnon transport signal is simultaneously measured at the detector via the lock-in amplifier. Additionally, we measure the DC spin pumping signal $V_{\mathrm{SP}}$ at the detector via a nanovoltmeter. (b) Magnetic field orientation dependent measurement of the magnon transport signal $V_{\mathrm{ac}}$ without any microwave excitation of the sample. Maximum signal is expected for $\varphi = \pm 180°, 0°$. (c) Magnon transport signal $V_{\mathrm{ac}}$ (black line) and spin pumping voltage $V_{\mathrm{SP}}$ (red line) as a function of the magnetic field strength. The field is pointing perpendicular to the Pt strips, corresponding to $\varphi = -180°$ and $0°$, respectively. In addition to the AC injector current, a microwave with frequency $f_{\mathrm{RF}} = 9\,\mathrm{GHz}$ and power $P_{\mathrm{RF}} \approx 0.3\,\mathrm{W}$ is applied to the CPW via the VNA.

In Fig. S17 (a) the full experimental setup including the electrical connections is schematically shown. For the magnon transport measurements, we used a YIG/Pt heterostructure with a YIG thickness of 2 µm. Two Pt strips with edge-to-edge distance of 200 nm, a width of 500 nm and a thickness of 7 nm are structured on top of the film. The sample with a substrate thickness of 1 mm is placed substrate-side down onto a RF stripline with center conductor width $w_{\mathrm{CPW}} = 1\,\mathrm{mm}$ such that the waveguide is oriented perpendicularly to the Pt strips. Simultaneously, we apply a static magnetic field pointing also perpendicularly to the Pt strips, which defines the magnetic field orientation $\varphi = 0°$.

In a first step, similar to the measurements presented in the main text, we apply a low frequency ($f = 13\,\mathrm{Hz}$) AC current $I_{\mathrm{ac}} = 100\,\mu\mathrm{A}$ to one strip (the injector) and measure the first harmonic response $V_{\mathrm{ac}}$ at the second strip (the detector) via a lock-in detection. Without applying any microwave signal to the CPW, we first measure the magnon transport signal at the detector as a function of the static magnetic field orientation $\varphi$. For this we choose a magnetic field strength of $\mu_0 H = 238\,\mathrm{mT}$, which approximately corresponds to the ferromagnetic resonance field of the YIG film for a microwave frequency of $f_{\mathrm{RF}} = 9\,\mathrm{GHz}$ (which we use for the FMR experiments in the next steps). Figure S17 (b) shows the magnetic field orientation dependent measurement of the detector signal $V_{\mathrm{ac}}$. As expected, we find the typical 180°-symmetric modulation of the signal [S15]. Note, that we expect the maximum signal for $\varphi = \pm 180°$ and $\varphi = 0°$. For $\varphi = -90°$ and $\varphi = 90°$, where we would not expect any finite signal, we find an offset signal of $\sim 60\,\mathrm{nV}$. This, however, was also observed for the sample discussed in the main text and does not affect the further interpretation of the measurements.

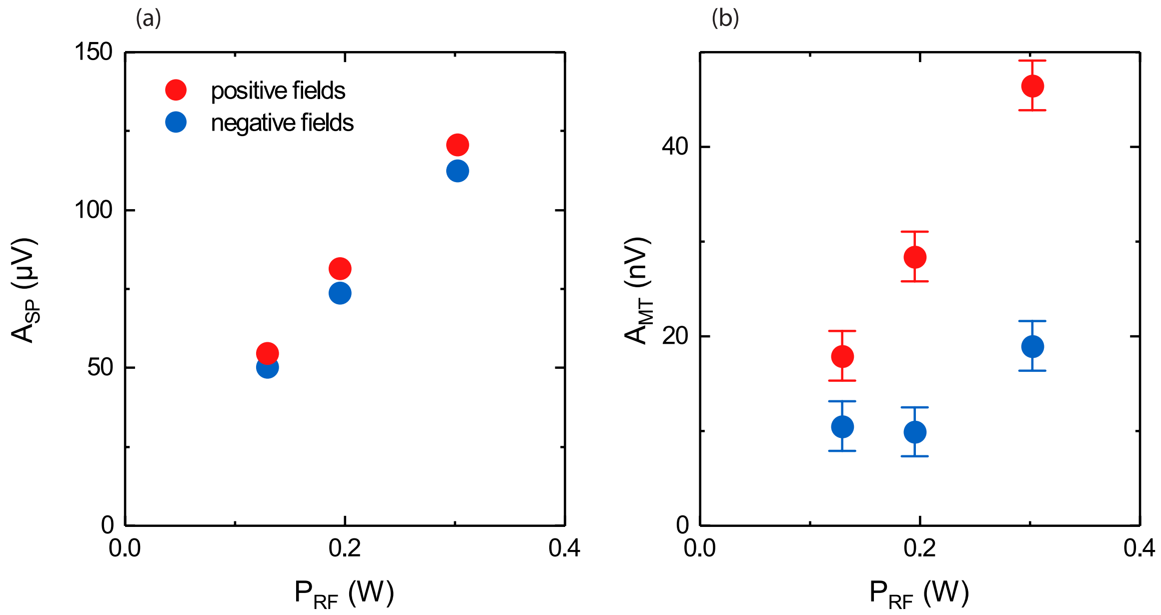


FIG. S18. (a) Spin pumping amplitude $A_{\mathrm{SP}}$ as a function of the microwave power $P_{\mathrm{RF}}$. A linear relation for both the positive and negative fields is observed. (b) Magnon transport modulation $A_{\mathrm{MT}}$ as a function of microwave power for both field directions.

As a next experiment, in addition to the low frequency AC injector current, we apply a microwave signal with frequency $f_{\mathrm{RF}} = 9\,\mathrm{GHz}$ and power $P_{\mathrm{RF}} \approx 0.3\,\mathrm{W}$ to the RF stripline using a vector network analyzer (VNA). In order to excite the FMR, we fix the external magnetic field to the direction oriented perpendicular to the Pt strips, i.e. $\varphi = -180°, 0°$. We then measure the magnon transport signal $V_{\mathrm{ac}}$ and the spin pumping signal $V_{\mathrm{SP}}$ via the lock-in amplifier and the DC nanovoltmeter simultaneously at the detector, respectively. In Fig. S17 (c), we plot $V_{\mathrm{ac}}$ (black line) and $V_{\mathrm{SP}}$ (red line) as a function of the magnetic field strength. The spin pumping signal $V_{\mathrm{SP}}$ exhibits the expected signature, showing a clear peak (dip) at the positive (negative) resonance field of approximately $|\mu_0 H| = 240\,\mathrm{mT}$. Note, that the difference between the baseline of the spin pumping voltage for positive and negative magnetic fields is attributed to the finite spin Seebeck signal due to the microwave heating of the sample. As expected, the baseline of the magnon transport signal $V_{\mathrm{ac}}$ lies at the voltage level of the rotation at $\varphi = \pm 180°, 0°$. More interestingly, however, the magnon transport signal $V_{\mathrm{ac}}$ also shows a clear peak structure at the resonance fields for both field directions. Moreover, these peaks do also agree with the peak/dip position of the spin pumping signal. We additionally observe that there is an asymmetry between the two peaks of the magnon transport signal [S31]. Comparing these peaks to the magnetization orientation dependent measurement in Fig. S17 (b), we find that the peaks correspond to a reduction

of the magnon transport signal. Following the model put forward in Ref. S2, we naively would have expected an increase of the signal. This is because the resonant excitation of the magnetization can be viewed as an effective increase of the magnon density in the YIG, which should result in an increase of the magnon conductivity. The fact, that our experiment shows the exact opposite behaviour might suggest an increase of scattering of the magnons from the injector with the collective mode excited via the FMR as reported in Ref. S31. This experiment might therefore be an indication of the fundamental difference between the incoherent magnon excitation via spin torque (as conducted in the main text) and the coherent excitation of the magnetization via FMR.

Finally, we want to adress the microwave power dependence of the spin pumping and magnon transport signal. To this end, we measured fieldsweeps of $V_{\mathrm{ac}}$ and $V_{\mathrm{SP}}$ (similar to Fig. S17 (c)) for three different microwave powers. Therafter, we extract the peak/dip amplitudes $A_{\mathrm{SP}}$ and $A_{\mathrm{MT}}$ for both the spin pumping and magnon transport signal for the different microwave powers, respectively (as indicated in Fig. S17 (c)). In Fig. S18 (a) we plot the spin pumping amplitude $A_{\mathrm{SP}}$ as a function of the microwave power for positive and negative fields separately. As expected, we find a linear relation of the spin pumping signal for both field directions [S3, S32–S34]. Panel (b) of Fig. S18 shows the peak amplitude $A_{\mathrm{MT}}$ of the magnon transport signal as a function of $P_{\mathrm{RF}}$ for both field directions. For positive fields (red points), we again find a linear relation between the FMR induced modulation of the magnon transport signal and the microwave power. For negative fields (blue points), the quantitative trend is not clear from the current data, but this might be attributed to the fact that the peak amplitudes for these low microwave powers are close to noise level of the measurement setup. At all microwave powers, the magnon transport signal is reduced, contrary to the DC current experiments discussed in the main text. We note that all microwave powers used in Fig. S18 correspond to driving fields in the non-linear regime. The SNR of our measurements did not allow to conclusively determine whether FMR in the linear regime affects the magnon transport characteristics.

---


[S1] K. Ganzhorn, S. Klingler, T. Wimmer, S. Geprägs, R. Gross, H. Huebl, and S. T. B. Goennenwein, Applied Physics Letters **109**, 022405 (2016).

[S2] L. J. Cornelissen, J. Liu, B. J. van Wees, and R. A. Duine, Physical Review Letters **120**, 097702 (2018).

[S3] Y. Tserkovnyak, A. Brataas, and G. E. W. Bauer, Physical Review Letters **88**, 117601 (2002).

[S4] W. Zhang, W. Han, X. Jiang, S.-H. Yang, and S. S. P. Parkin, Nature Physics **11**, 496 (2015).

[S5] Y. Tserkovnyak, A. Brataas, and G. E. W. Bauer, Physical Review B **66**, 224403 (2002).

[S6] M. Zwierzycki, Y. Tserkovnyak, P. J. Kelly, A. Brataas, and G. E. W. Bauer, Physical Review B **71**, 064420 (2005).

[S7] E. Barati, M. Cinal, D. M. Edwards, and A. Umerski, Physical Review B **90**, 014420 (2014).

[S8] J. Xiao, G. E. W. Bauer, K.-c. Uchida, E. Saitoh, and S. Maekawa, Physical Review B **81**, 214418 (2010).

[S9] S. A. Bender, R. A. Duine, A. Brataas, and Y. Tserkovnyak, Physical Review B **90**, 094409 (2014).

[S10] With increasing temperature difference $\delta T$, the critical current is always shifted to higher values, independent of the actual sign of $\delta T$ (see Ref. [S9]).

[S11] M. Schreier, A. Kamra, M. Weiler, J. Xiao, G. E. W. Bauer, R. Gross, and S. T. B. Goennenwein, Physical Review B **88**, 094410 (2013).

[S12] N. Thiery, V. V. Naletov, L. Vila, A. Marty, A. Brenac, J.-F. Jacquot, G. de Loubens, M. Viret, A. Anane, V. Cros, J. Ben Youssef, N. Beaulieu, V. E. Demidov, B. Divinskiy, S. O. Demokritov, and O. Klein, Physical Review B **97**, 064422 (2018).

[S13] N. Thiery, A. Draveny, V. V. Naletov, L. Vila, J. P. Attané, C. Beigné, G. de Loubens, M. Viret, N. Beaulieu, J. Ben Youssef, V. E. Demidov, S. O. Demokritov, A. N. Slavin, V. S. Tiberkevich, A. Anane, P. Bortolotti, V. Cros, and O. Klein, Physical Review B **97**, 060409 (2018).

[S14] L. J. Cornelissen and B. J. van Wees, Physical Review B **93**, 020403 (2016).

[S15] L. J. Cornelissen, J. Liu, R. A. Duine, J. B. Youssef, and B. J. van Wees, Nature Physics **11**, 1022 (2015).

[S16] L. J. Cornelissen, K. J. H. Peters, G. E. W. Bauer, R. A. Duine, and B. J. van Wees, Physical Review B **94**, 014412 (2016).

[S17] X.-G. Wang, Z.-W. Zhou, Y.-Z. Nie, Q.-L. Xia, and G.-H. Guo, Physical Review B **97**, 094401 (2018).

[S18] This is indeed not very surprising, since we use a double layer resist system for structuring the Pt strips via a lift-off procedure. Thereby, we ensure are larger undercut of the structured resists, which in turn yields better results regarding the lift-off. As a compromise we loose some resolution, which explains the slightly larger strip width determined via the AFM measurements.

[S19] H. H. Landault and R. Boernstein, *Part A: Garnets and Perovskites*, edited by K.-H. Hellwege and A. M. Hellwege (Springer-Verlag, 1978).

[S20] Note, that the amplitudes in these calculations correspond to the root mean squared voltage that was measured via the lock in amplifier. The amplitudes and voltage levels given in the main text are multiplied by a factor of $\sqrt{2}$ to present the peak voltages.

[S21] J. Shan, L. J. Cornelissen, N. Vlietstra, J. Ben Youssef, T. Kuschel, R. A. Duine, and B. J. van Wees, Phys. Rev. B **94**, 174437 (2016).

[S22] B. Flebus, S. A. Bender, Y. Tserkovnyak, and R. A. Duine, Phys. Rev. Lett. **116**, 117201 (2016).

[S23] A. Hamadeh, O. d'Allivy Kelly, C. Hahn, H. Meley, R. Bernard, A. H. Molpeceres, V. V. Naletov, M. Viret, A. Anane, V. Cros, S. O. Demokritov, J. L. Prieto, M. Muñoz, G. de Loubens, and O. Klein, Physical Review Letters **113**, 197203 (2014).

[S24] M. Collet, X. de Milly, O. d'Allivy Kelly, V. V. Naletov, R. Bernard, P. Bortolotti, J. B. Youssef, V. E. Demidov, S. O. Demokritov, J. L. Prieto, M. Muñoz, V. Cros, A. Anane, G. de Loubens, and O. Klein, Nature Communications **7**, 10377 (2016).

[S25] B. Hillebrands and A. Thiaville, eds., *Spin Dynamics in Confined Magnetic Structures III* (Springer Berlin Heidelberg, 2006).

[S26] D. D. Stancil and A. Prabhakar, *Spin Waves* (Springer US, 2009).

[S27] Y.-T. Chen, S. Takahashi, H. Nakayama, M. Althammer, S. T. B. Goennenwein, E. Saitoh, and G. E. W. Bauer, Physical Review B **87**, 144411 (2013).

[S28] S. S.-L. Zhang and S. Zhang, Physical Review B **86**, 214424 (2012).

[S29] S. T. B. Goennenwein, R. Schlitz, M. Pernpeintner, K. Ganzhorn, M. Althammer, R. Gross, and H. Huebl, Applied Physics Letters **107**, 172405 (2015).

[S30] M. Althammer, S. Meyer, H. Nakayama, M. Schreier, S. Altmannshofer, M. Weiler, H. Huebl, S. Geprägs, M. Opel, R. Gross, D. Meier, C. Klewe, T. Kuschel, J.-M. Schmalhorst, G. Reiss, L. Shen, A. Gupta, Y.-T. Chen, G. E. W. Bauer, E. Saitoh, and S. T. B. Goennenwein, Physical Review B **87**, 224401 (2013).

[S31] J. Liu, F. Feringa, B. Flebus, L. J. Cornelissen, J. C. Leutenantsmeyer, R. A. Duine, and B. J. van Wees, Phys. Rev. B **99**, 054420 (2019).

[S32] K. Ando, J. Ieda, K. Sasage, S. Takahashi, S. Maekawa, and E. Saitoh, Applied Physics Letters **94**, 262505 (2009).

[S33] M. V. Costache, M. Sladkov, S. M. Watts, C. H. van der Wal, and B. J. van Wees, Physical Review Letters **97**, 216603 (2006).

[S34] F. D. Czeschka, L. Dreher, M. S. Brandt, M. Weiler, M. Althammer, I.-M. Imort, G. Reiss, A. Thomas, W. Schoch, W. Limmer, H. Huebl, R. Gross, and S. T. B. Goennenwein, Physical Review Letters **107**, 046601 (2011).
